# Supplementary material for: FlowCapX: Physics-Grounded Flow Capture with Long-Term Consistency
Source: arXiv:2510.23122 source file (2025-10-27)
Supplement: Supplementary file 1 [file appendix.tex]

\section{Appendix}

\subsection{Extended Experimental Results}

\begin{figure}[bp]
    \centering
    \begin{minipage}[t]{\linewidth}
        \centering
        \begin{minipage}[t]{0.5\linewidth}
            %\centering
            \includegraphics[width=\linewidth]{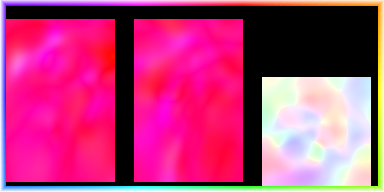}
            \vspace{-1.9em}
            \caption*{PINF}
            \includegraphics[width=\linewidth]{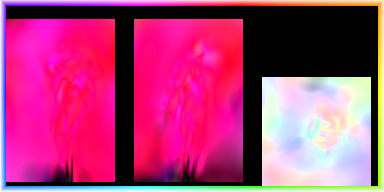}
            \vspace{-1.9em}
            \caption*{PICT}

        \end{minipage}%
        \hfill
        \begin{minipage}[t]{0.5\textwidth}
            \centering
            \includegraphics[width=\textwidth]{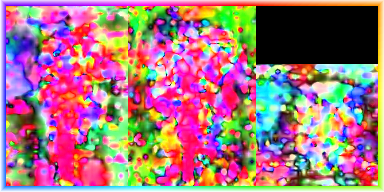}
            \vspace{-1.9em}
            \caption*{HyFluid}
            
            \includegraphics[width=\textwidth]{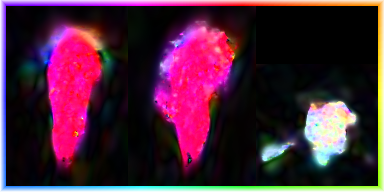}
            \vspace{-1.9em}
            \caption*{Ours}
        \end{minipage}
    \end{minipage}
    \vspace{-6pt}
    \caption{The velocity visualization on the ScalarFlow scene. Compared to PINF and PICT, which miss turbulent structures, and HyFluid, which generates excessive chaos, our method achieves a balanced reconstruction with physical plausibility and detailed turbulence.}
    \label{fig:velcmpScalar}
\end{figure}

\begin{figure}[hbp]
    \centering
    \begin{minipage}[t]{\linewidth}
        \centering
        \begin{minipage}[t]{\linewidth}
            \centering
            
            % \vspace{-20pt}
            \includegraphics[width=\textwidth]{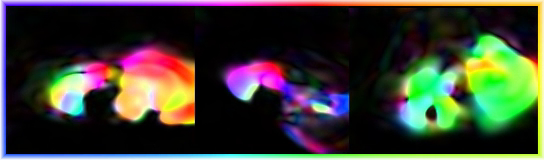}
            % \vspace{-34pt}
            \vspace{-1.9em}
            \caption*{\textcolor{black}{Ours (Coarse-level)}}
            
            \includegraphics[width=\textwidth]{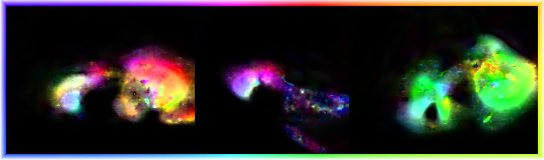}
            % \vspace{-34pt}
            \vspace{-1.9em}
            \caption*{\textcolor{black}{Ours (Full)}}
            
            \includegraphics[width=\textwidth]{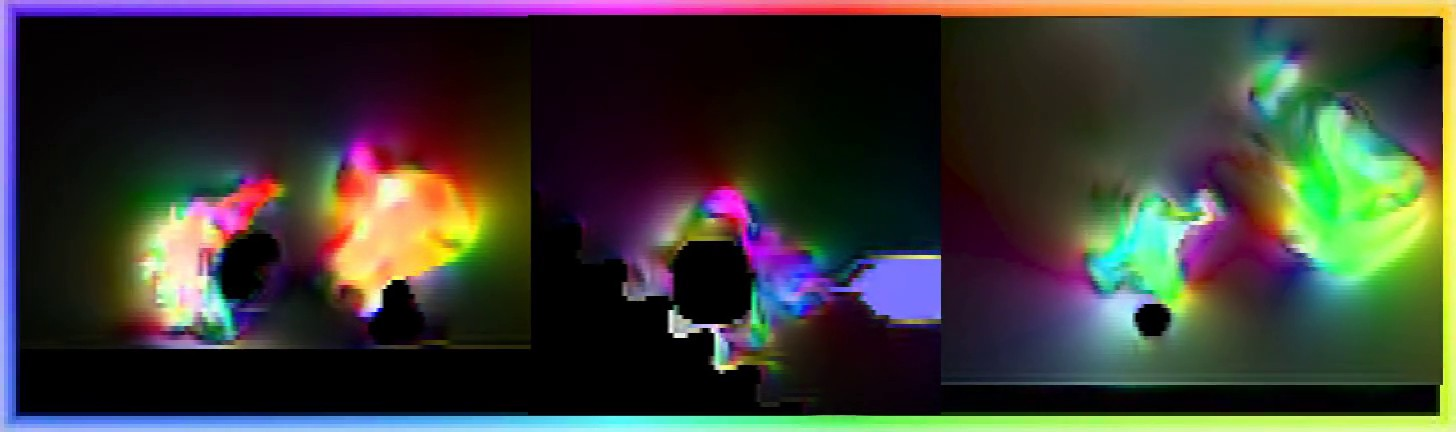}
            % \vspace{-34pt}
            \vspace{-1.9em}
            \caption*{\textcolor{black}{Ground Truth}}
        \end{minipage}
    \end{minipage}
    \vspace{-6pt}
    \caption{Velocity visualization on the Game scene. The results demonstrate that our method accurately reconstructs the velocity field, closely matching the ground truth. They also validate the effectiveness of our hybrid framework, in which the coarse level captures the global structure, and the fine level resolves high-frequency details.}
    \label{fig:velcmpGame}
\end{figure}
\paragraph{Velocity field visualization} Beyond the velocity visualization results on Cylinder and ScalarSyn in main paper, Fig.~\ref{fig:velcmpScalar} presents the velocity visualization result on ScalarFlow, where only our method reconstructs a physically plausible velocity field while effectively preserving turbulent details. Furthermore, to evaluate the scalability of our approach, we apply it to the Game scene proposed by~\citet{chu2022physics}. As shown in Fig.~\ref{fig:velcmpGame} and Fig.~\ref{fig:game}, our method is also able to reconstruct the velocity field in this large-scale scene.

\begin{figure*}[htbp]
    \centering
    \begin{subfigure}{0.32\linewidth}
        \newcommand{\formattedgraphics}[1]{\includegraphics[trim=0cm 3pt 0cm 0cm,clip,width=\linewidth]{#1}}
    	\centering
    	\formattedgraphics{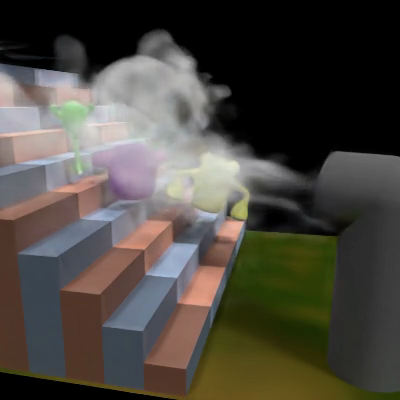}
    	% \caption{density}
            \vspace{-2ex}
    	\label{fig:game-density}
        
    \end{subfigure}
    \hspace{-2ex}
    \begin{subfigure}{0.32\linewidth}
        \newcommand{\formattedgraphics}[1]{\includegraphics[trim=0cm 180pt 0cm 20pt, clip,width=\linewidth]{#1}}
    	\centering
    	\formattedgraphics{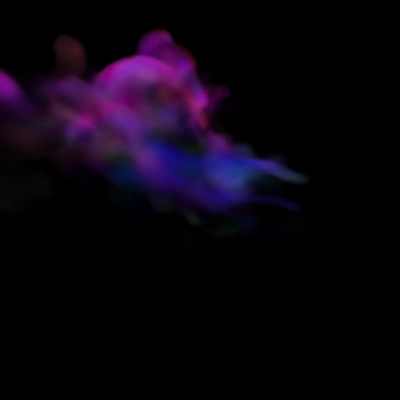}\\
        \vspace{-0.1cm}
    	\formattedgraphics{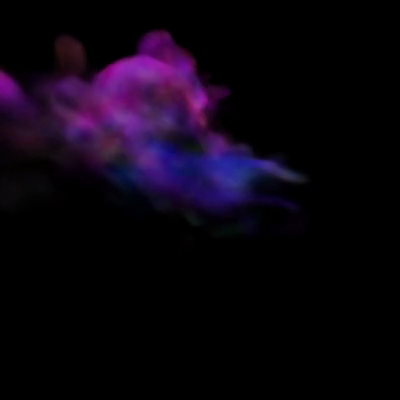}
    	% \caption{velocity}
            \vspace{-2ex}
    	\label{fig:game-velocity}
    \end{subfigure}
    \hspace{-2ex}
    \begin{subfigure}{0.32\linewidth}
        \newcommand{\formattedgraphics}[1]{\includegraphics[trim=0cm 180pt 0cm 20pt, clip,width=\linewidth]{#1}}
    	\centering
    	\formattedgraphics{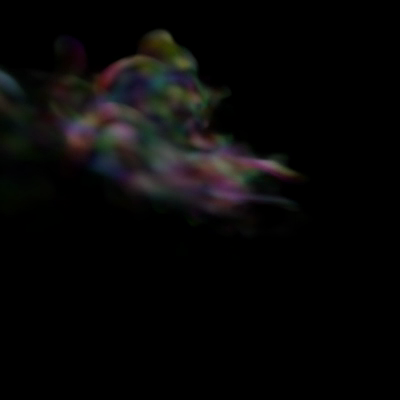}\\
        \vspace{-0.1cm}
    	\formattedgraphics{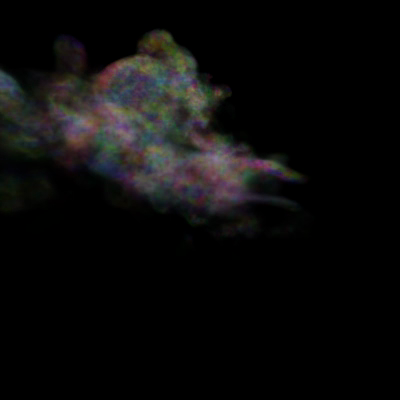}
    	% \caption{vorticity}
            \vspace{-2ex}
    	\label{fig:game-vorticity}
    \end{subfigure}
 \caption{Visualization of the reconstructed results on the Game scene. The leftmost column shows the rendered results of the reconstructed dynamic density and static boundary. The middle column displays volume renderings of the coarse-level velocity and full velocity from top to bottom, while the rightmost column presents volume renderings of the coarse-level vorticity and full vorticity from top to bottom. These results demonstrate that our method is applicable to complex scenarios and highlight how the coarse-level velocity captures the overall structure of the velocity field, while the fine-level velocity preserves the detailed features. } 
 % \vspace{-3ex}
  \label{fig:game}
\end{figure*}

\paragraph{Re-simulation} In addition to the visual results and the peak signal-noise ratio (PSNR) comparisons presented in the main paper, we provide a more comprehensive quantitative evaluation in Table~\ref{tbl:resim}, including structural similarity index measure (SSIM) and the perceptual metric LPIPS~\cite{zhang2018unreasonable}. Our method achieves competitive results on the re-simulation task, performing consistently well in the Cylinder scene across all metrics and obtaining comparable PSNR and SSIM scores on the ScalarSyn and ScalarFlow datasets. While LPIPS values are slightly higher than those reported by some baselines, this likely reflects a trade-off favoring data fidelity. Overall, the results suggest that our approach performs comparably to existing methods across different re-simulation scenarios.

\begin{table*}[htbp]
\centering
\small
\begin{tabular}{lccccccccc}
\toprule
\multirow{2}{*}{Model} & \multicolumn{3}{c}{Cylinder} & \multicolumn{3}{c}{ScalarSyn} & \multicolumn{3}{c}{ScalarFlow} \\
\cmidrule(lr){2-4} \cmidrule(lr){5-7} \cmidrule(lr){8-10}
 & PSNR$\uparrow$ & SSIM$\uparrow$ & LPIPS$\downarrow$ & PSNR$\uparrow$ & SSIM$\uparrow$ & LPIPS$\downarrow$ & PSNR$\uparrow$ & SSIM$\uparrow$ & LPIPS$\downarrow$ \\
\midrule
PINF    & 23.04 & 0.8712 & 0.2017 & 30.06 & 0.9225 & \textbf{0.08284} & 31.24 & \textbf{0.9635} & 0.1020 \\
PICT    & \underline{26.74} & \underline{0.9148} & \underline{0.1675} & 31.00 & 0.8998 & 0.1000 & 31.97 & 0.9490 & \underline{0.09932} \\
HyFluid & --        & --     & --       & \underline{32.41}   & \textbf{0.9340} & \underline{0.08536} & \underline{32.62} & 0.9555 & \textbf{0.08186} \\
Ours    & \textbf{28.68} & \textbf{0.9337} & \textbf{0.1422} & \textbf{32.91} & \underline{0.9230} & 0.09686 & \textbf{33.28} & \underline{0.9576} & 0.1001 \\
\bottomrule
\end{tabular}

% \vspace{-0.5em}
% \footnotesize \textbf{Note}: Cylinder scene excludes HyFluid due to obstacle limitations. ScalarFlow only evaluates divergence due to lack of velocity and density ground truth.
\caption{Quantitative re-simulation comparisons on Cylinder, ScalarSyn, and ScalarFlow datasets. Our method consistently outperforms all baselines in the Cylinder scene across all metrics, demonstrating strong generalization in flow scenarios with obstacles. On ScalarSyn and ScalarFlow, we achieve the best or comparable PSNR and SSIM scores. While our LPIPS values are slightly higher than some baselines (e.g., HyFluid), this can be attributed to a trade-off, as our approach prioritizes data fidelity during reconstruction, which may lead to minor compromises in perceptual similarity. Overall, these results show that our method is robust and competitive across diverse re-simulation tasks.}
\label{tbl:resim}
\end{table*}

\paragraph{Prediction} We also conduct the prediction task proposed by~\citet{yu2024inferring}, where the reconstructed velocity field is evolved using a standard grid-based fluid simulation framework~\cite{mantaflow}. As shown in Fig.~\ref{fig:predReal}, both the baselines and our method continue to exhibit a significant discrepancy with the Ground Truth. Nevertheless, our approach demonstrates relatively more turbulent details compared to PINF and PICT, and produces a global structure more aligned with the Ground Truth than HyFluid.

It is worth noting that this prediction task selects an arbitrary frame of the reconstructed velocity field for forward simulation. Due to this sensitivity, the task may not serve as a reliable indicator of reconstruction quality. We report it here for completeness and comparison, but note that the large performance variation and overall low accuracy across all methods suggest its limitations as a robust evaluation metric.

\begin{figure*}[thp]
    \centering
    \setlength{\imagewidth}{0.2\textwidth}
      \newcommand{\formattedgraphics}[2]{%
        \begin{tikzpicture}
        \clip (0, 5pt) rectangle (\imagewidth, 120pt); 
          \node[anchor=south west, inner sep=0] at (0,0){\includegraphics[width=\imagewidth]{#1}};
          %\draw[red] (0.25\imagewidth, 0.2\imagewidth) rectangle (0.7\imagewidth, 0.65\imagewidth);
          \node[anchor=west,text=white] at (.01\imagewidth, 1.07\imagewidth) {\sffamily\footnotesize #2};
          \end{tikzpicture}%
      }
    \formattedgraphics{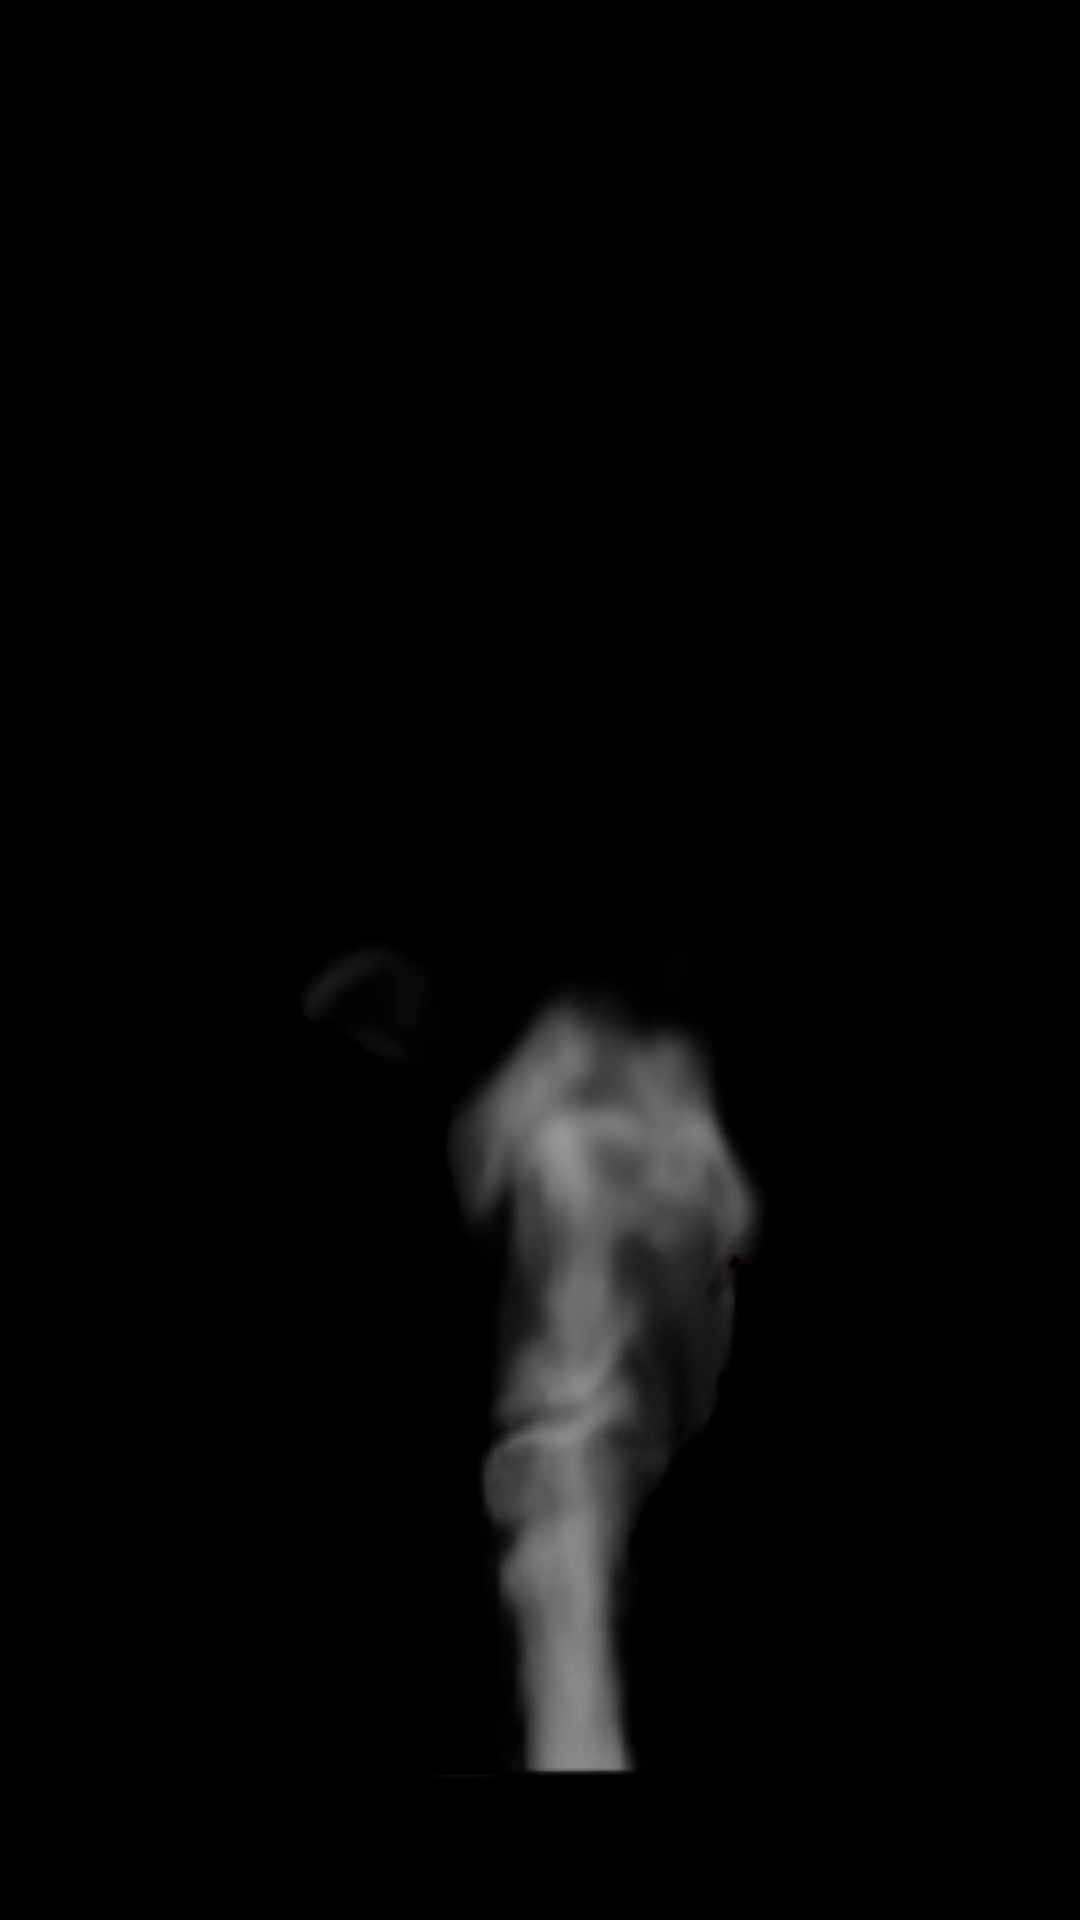}{PINF}%
    \hspace{-0.1cm}
    %\hfill
    \formattedgraphics{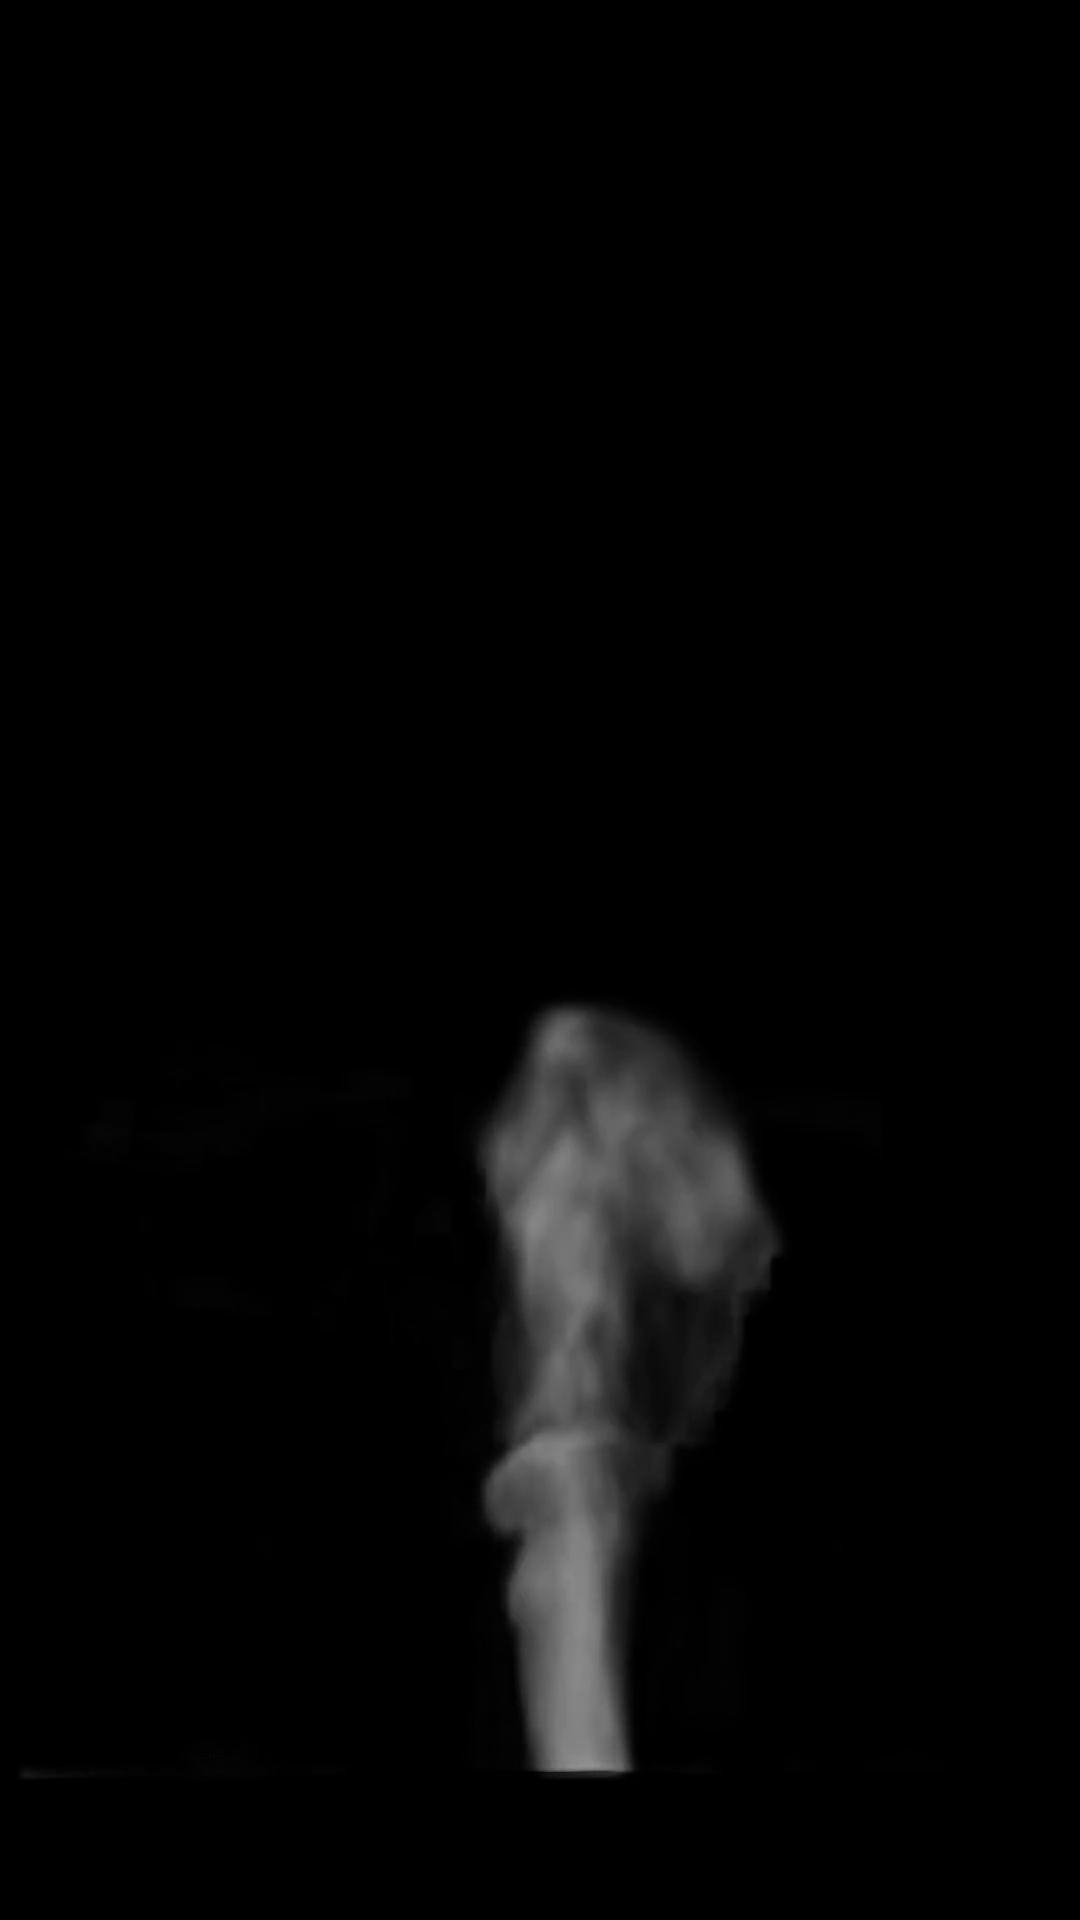}{PICT}%
    \hspace{-0.1cm}
    %\hfill
    \formattedgraphics{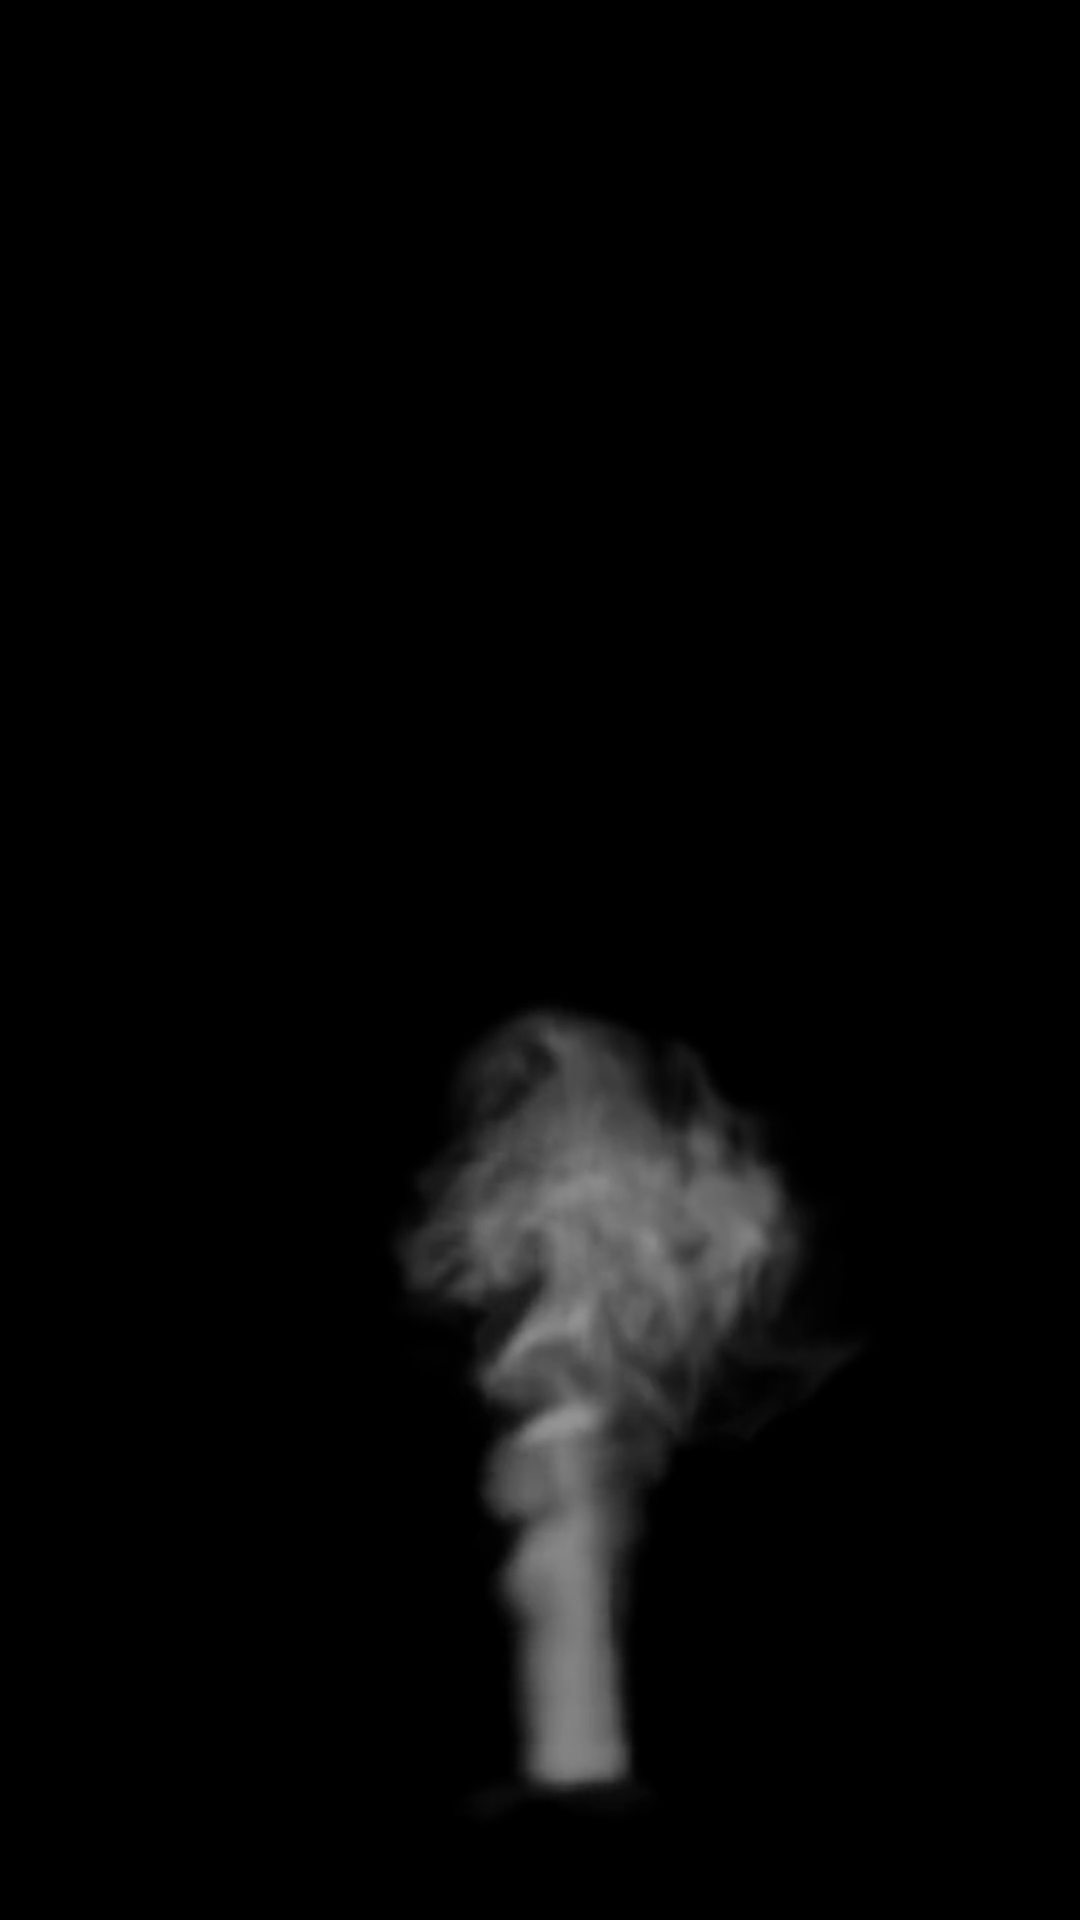}{HyFluid}%
    \hspace{-0.1cm}
    %\hfill
    \formattedgraphics{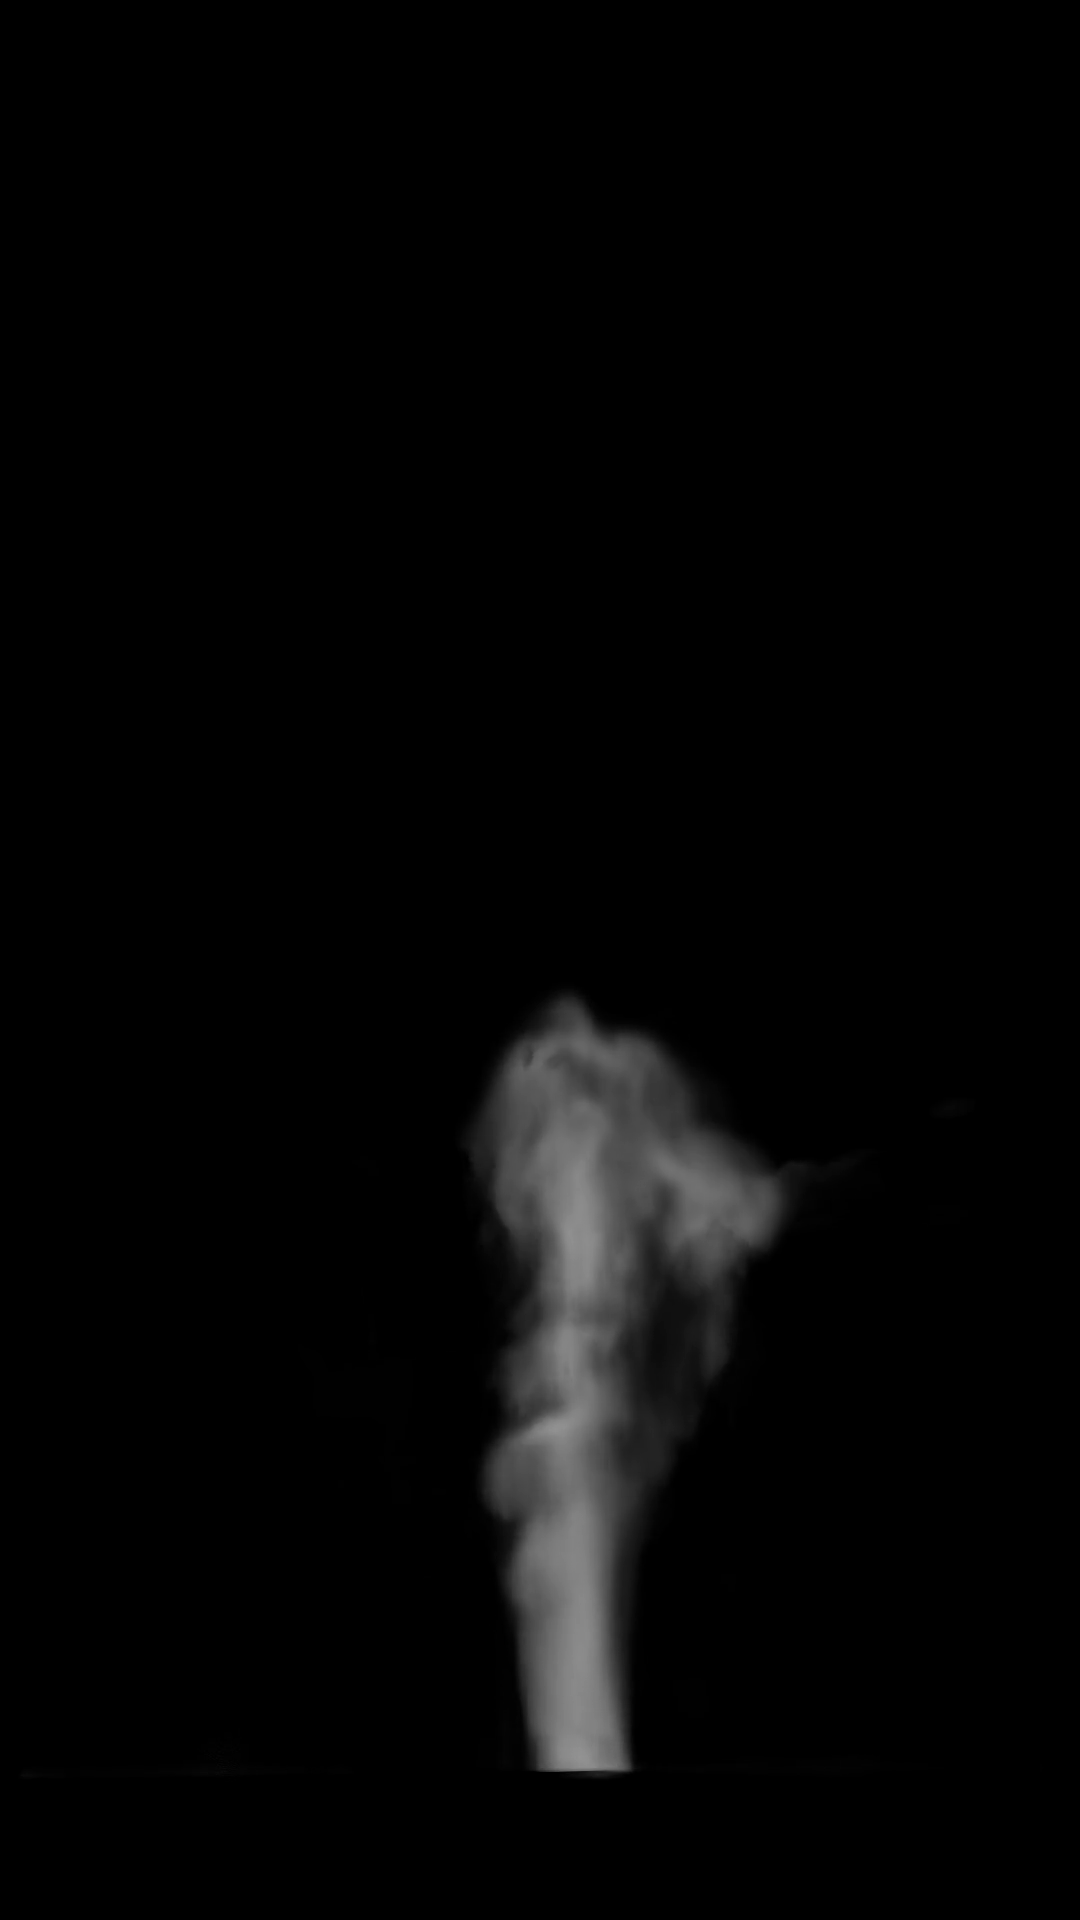}{Ours}%
    \hspace{-0.1cm}
    %\hfill
    \formattedgraphics{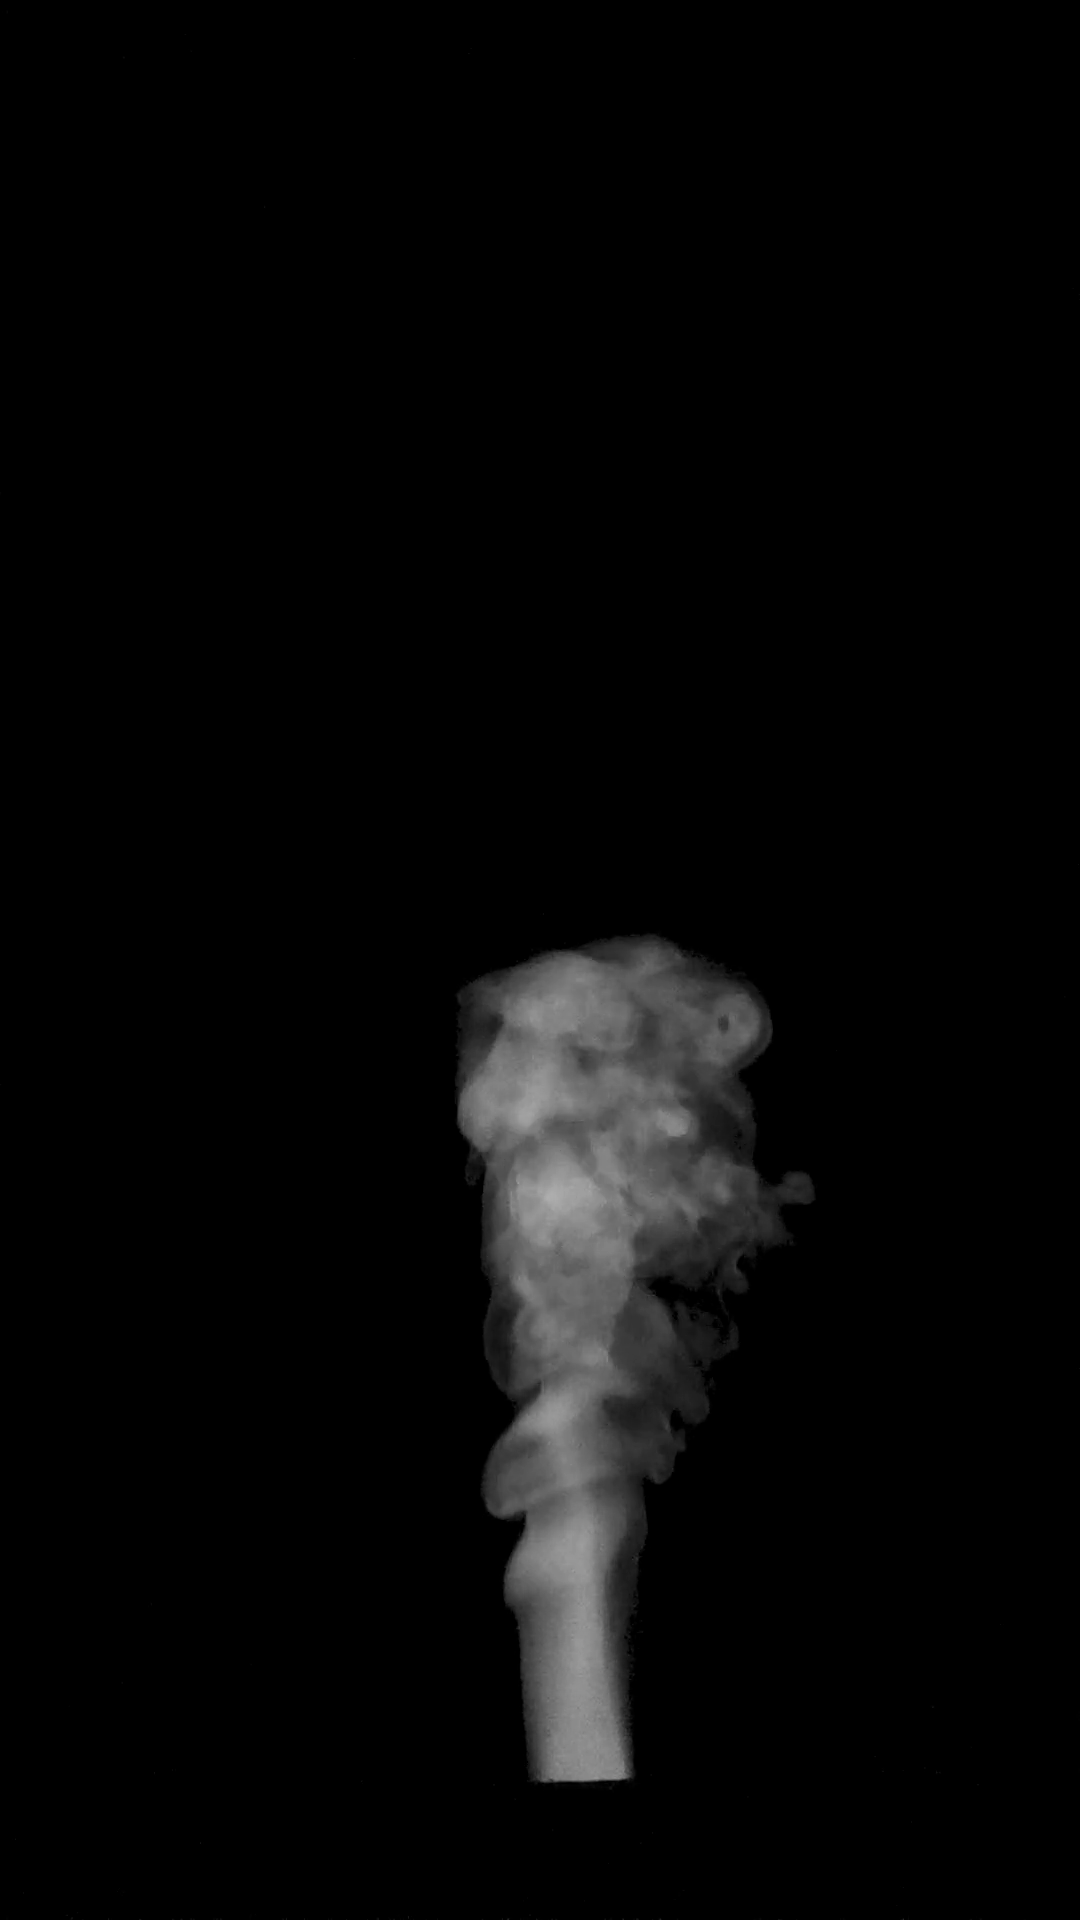}{Ground Truth}%
    \hspace{-0.1cm}
    \\
    % \vspace{-0.5em}
    \caption{Visualization of prediction results on the ScalarFlow dataset. All methods show notable deviations from the ground truth in this challenging prediction task. The velocity fields reconstructed by PINF and PICT tend to be overly smooth, resulting in a simplified upward motion of the smoke. HyFluid introduces more turbulence but suffers from structural inconsistencies. Our method captures finer vortex details and better preserves the overall flow structure, showing improved alignment with the ground truth.}
    \label{fig:predReal}
  \end{figure*}

\rv{
\subsection{Velocity Masking}
We also compare the velocity fields reconstructed by our method with those from baseline methods using a density-based mask. Specifically, the mask is defined as the spatial region where the density exceeds a prescribed threshold. It is worth noting that the choice of this threshold is highly parameter-dependent—simply using all non-zero density values as the mask does not necessarily yield good results. Instead, the density threshold must be carefully tuned for each scene to achieve satisfactory performance. We present results on the ScalarSyn dataset, which is the most representative; results on other datasets are available in our supplementary videos.

As illustrated in Fig.~\ref{fig:velcmp_thresh0} and Fig.~\ref{fig:velcmp_thresh1}, we use the ground-truth density to mask the velocity field, setting the density threshold to $0$ and $1$, respectively. With a small threshold such as $0$, the mask fails to accurately capture the shape of the velocity field. With a large threshold such as $1$, it causes some areas with non-zero velocity to be incorrectly set to zero. The results in Fig.~\ref{fig:tracerThresh0} and Fig.~\ref{fig:tracerThresh1} also support this observation: with a low threshold, paper pieces that should remain stationary are blown away, whereas with a high threshold, fewer are lifted compared to the ground truth. In contrast, by incorporating our boundary loss $\mathcal{L}_{\text{bnd}}$ and kinetic loss $\mathcal{L}_{\text{kine}}$, our method can automatically produce a reasonable velocity mask without manual tuning.
}

\begin{figure}[bp]
    \centering
    \begin{minipage}[t]{\linewidth}
        \centering
        \begin{minipage}[t]{0.5\linewidth}
            %\centering
            \includegraphics[width=\linewidth]{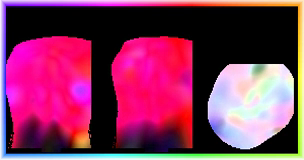}
            \vspace{-1.9em}
            \caption*{PINF}
            \includegraphics[width=\linewidth]{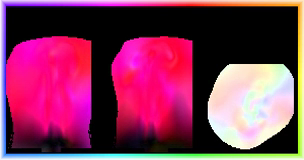}
            \vspace{-1.9em}
            \caption*{PICT}

        \end{minipage}%
        \hfill
        \begin{minipage}[t]{0.5\textwidth}
            \centering
            \includegraphics[width=\textwidth]{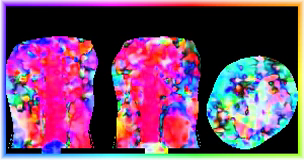}
            \vspace{-1.9em}
            \caption*{HyFluid}
            
            \includegraphics[width=\textwidth]{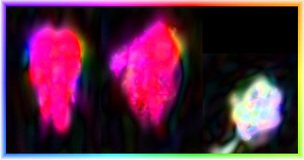}
            \vspace{-1.9em}
            \caption*{Ours}
        \end{minipage}
    \end{minipage}
     \begin{minipage}[t]{\linewidth}
        \centering
        \includegraphics[width=0.5\linewidth]{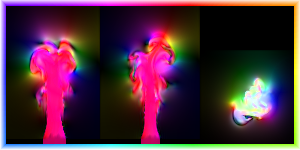}
        \vspace{-0.9em}
        \caption*{Ground Truth}
         
    \end{minipage}%
    \vspace{-6pt}
    \caption{\rv{Velocity visualization on the ScalarSyn scene, where the reconstructed velocity from baseline methods is masked using the ground truth density with a threshold of $0$. With such a small threshold, the mask fails to accurately capture the shape of the velocity field.}}
    \label{fig:velcmp_thresh0}
\end{figure}

\begin{figure}[bp]
    \centering
    \begin{minipage}[t]{\linewidth}
        \centering
        \begin{minipage}[t]{0.5\linewidth}
            %\centering
            \includegraphics[width=\linewidth]{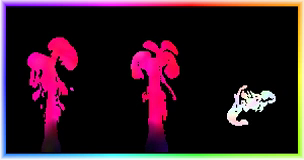}
            \vspace{-1.9em}
            \caption*{PINF}
            \includegraphics[width=\linewidth]{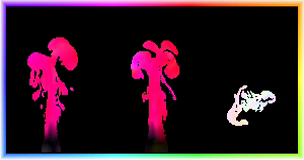}
            \vspace{-1.9em}
            \caption*{PICT}

        \end{minipage}%
        \hfill
        \begin{minipage}[t]{0.5\textwidth}
            \centering
            \includegraphics[width=\textwidth]{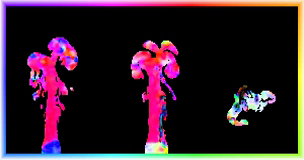}
            \vspace{-1.9em}
            \caption*{HyFluid}
            
            \includegraphics[width=\textwidth]{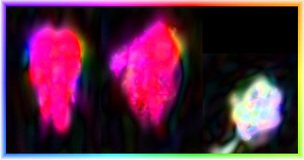}
            \vspace{-1.9em}
            \caption*{Ours}
        \end{minipage}
    \end{minipage}
     \begin{minipage}[t]{\linewidth}
        \centering
        \includegraphics[width=0.5\linewidth]{fig/Experiments/ScalarSyn_vel/gt27.png}
        \vspace{-0.9em}
        \caption*{Ground Truth}
         
    \end{minipage}%
    \vspace{-6pt}
    \caption{\rv{Velocity visualization on the ScalarSyn scene, where the reconstructed velocity from baseline methods is masked using the ground truth density with a threshold of $1$. From the visualization, a large threshold causes regions that should have non-zero velocity to be incorrectly set to zero.}}
    \label{fig:velcmp_thresh1}
\end{figure}

\begin{figure*}[htbp]
    \centering
    \setlength{\imagewidth}{0.2\textwidth}
      \newcommand{\formattedgraphics}[2]{%
        \begin{tikzpicture}%[spy using outlines={rectangle, magnification=2, connect spies}]
          \clip (0, 15pt) rectangle (\imagewidth, 140pt);
          \node[anchor=south west, inner sep=0] at (0,0){\includegraphics[width=\imagewidth,trim={3cm 0cm 3cm 7cm},clip]{#1}};
          %\spy [red,size=.41\imagewidth] on (0.65\imagewidth,1.05\imagewidth) in node at (0.25\imagewidth,.4\imagewidth);
          \node[anchor=west,text=white] at (.01\imagewidth, 1.27\imagewidth) {\sffamily\footnotesize #2};
          \end{tikzpicture}%
      }
      \newcommand{\mygraphics}[3]{%
        \begin{tikzpicture}[spy using outlines={rectangle, magnification=2, connect spies}]
          \clip (0, 15pt) rectangle (\imagewidth, 140pt);
          \node[anchor=south west, inner sep=0] at (0,0){\includegraphics[width=\imagewidth]{#1}};
          \spy [red,size=.41\imagewidth] on (0.65\imagewidth,1.05\imagewidth) in node at (0.25\imagewidth,.4\imagewidth);
          \node[anchor=west,text=white] at (.01\imagewidth, 1.29\imagewidth) {\sffamily\footnotesize #2};
          \node[anchor=west,text=white] at (0.01\imagewidth, 1.205\imagewidth) {\sffamily\scriptsize #3};%
          \end{tikzpicture}%
      }
    % \formattedgraphics{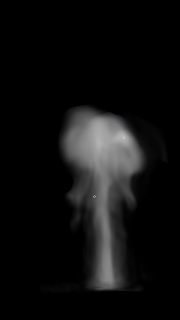}{PINF}%
    \formattedgraphics{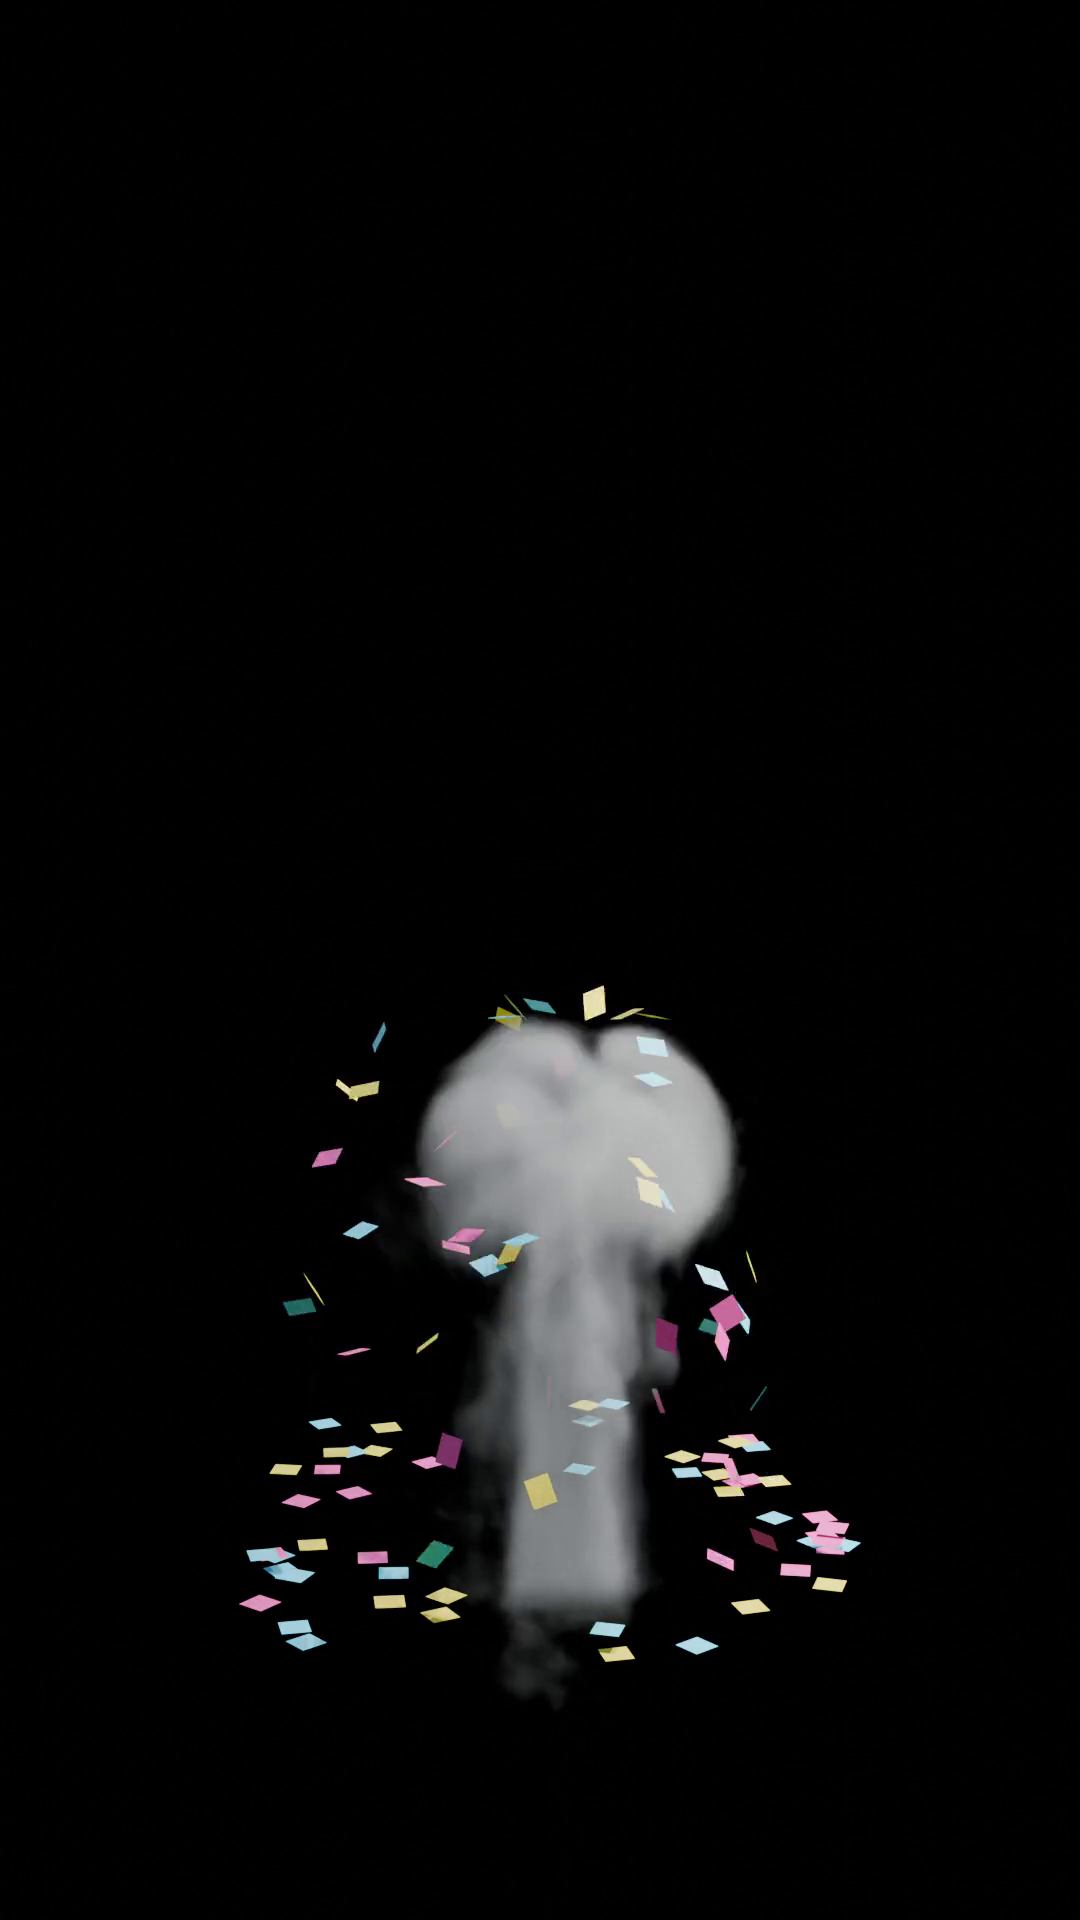}{\textbf{PINF}}
    \hspace{-0.18cm}
    % \hfill
    % \formattedgraphics{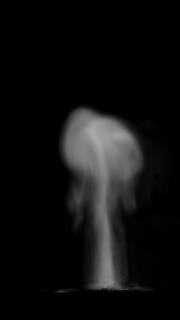}{PICT}%
    % \mygraphics{fig/Experiments/ScalarSyn_resim/pict_029.png}{\textbf{PICT}}{PSNR $31.00$}
    \formattedgraphics{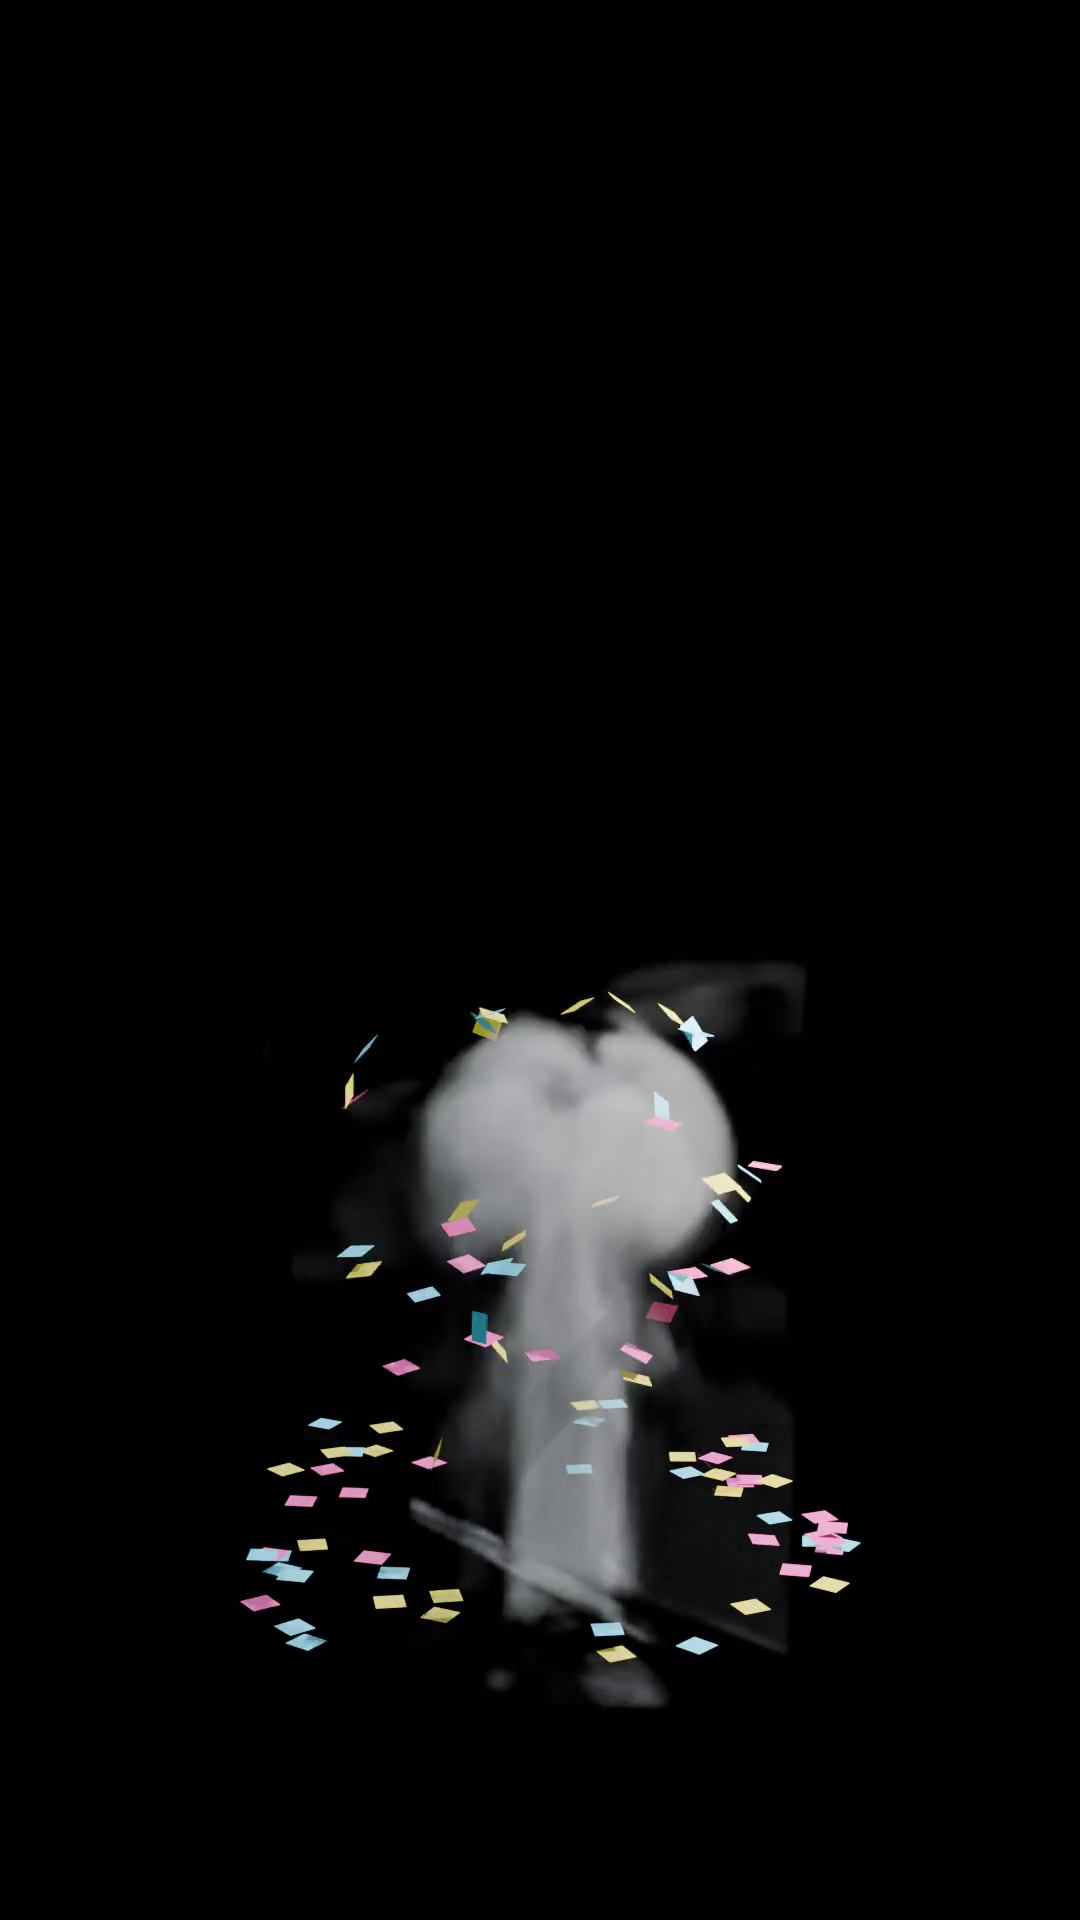}{\textbf{PICT}}
    \hspace{-0.18cm}
    % \hfill
    % \formattedgraphics{fig/Experiments/ScalarSyn_resim/HyFluid_rgb_029.png}{HyFluid}%
    % \mygraphics{fig/Experiments/ScalarSyn_resim/HyFluid_rgb_029.png}{\textbf{Hyfluid}}{PSNR $32.41$}
    \formattedgraphics{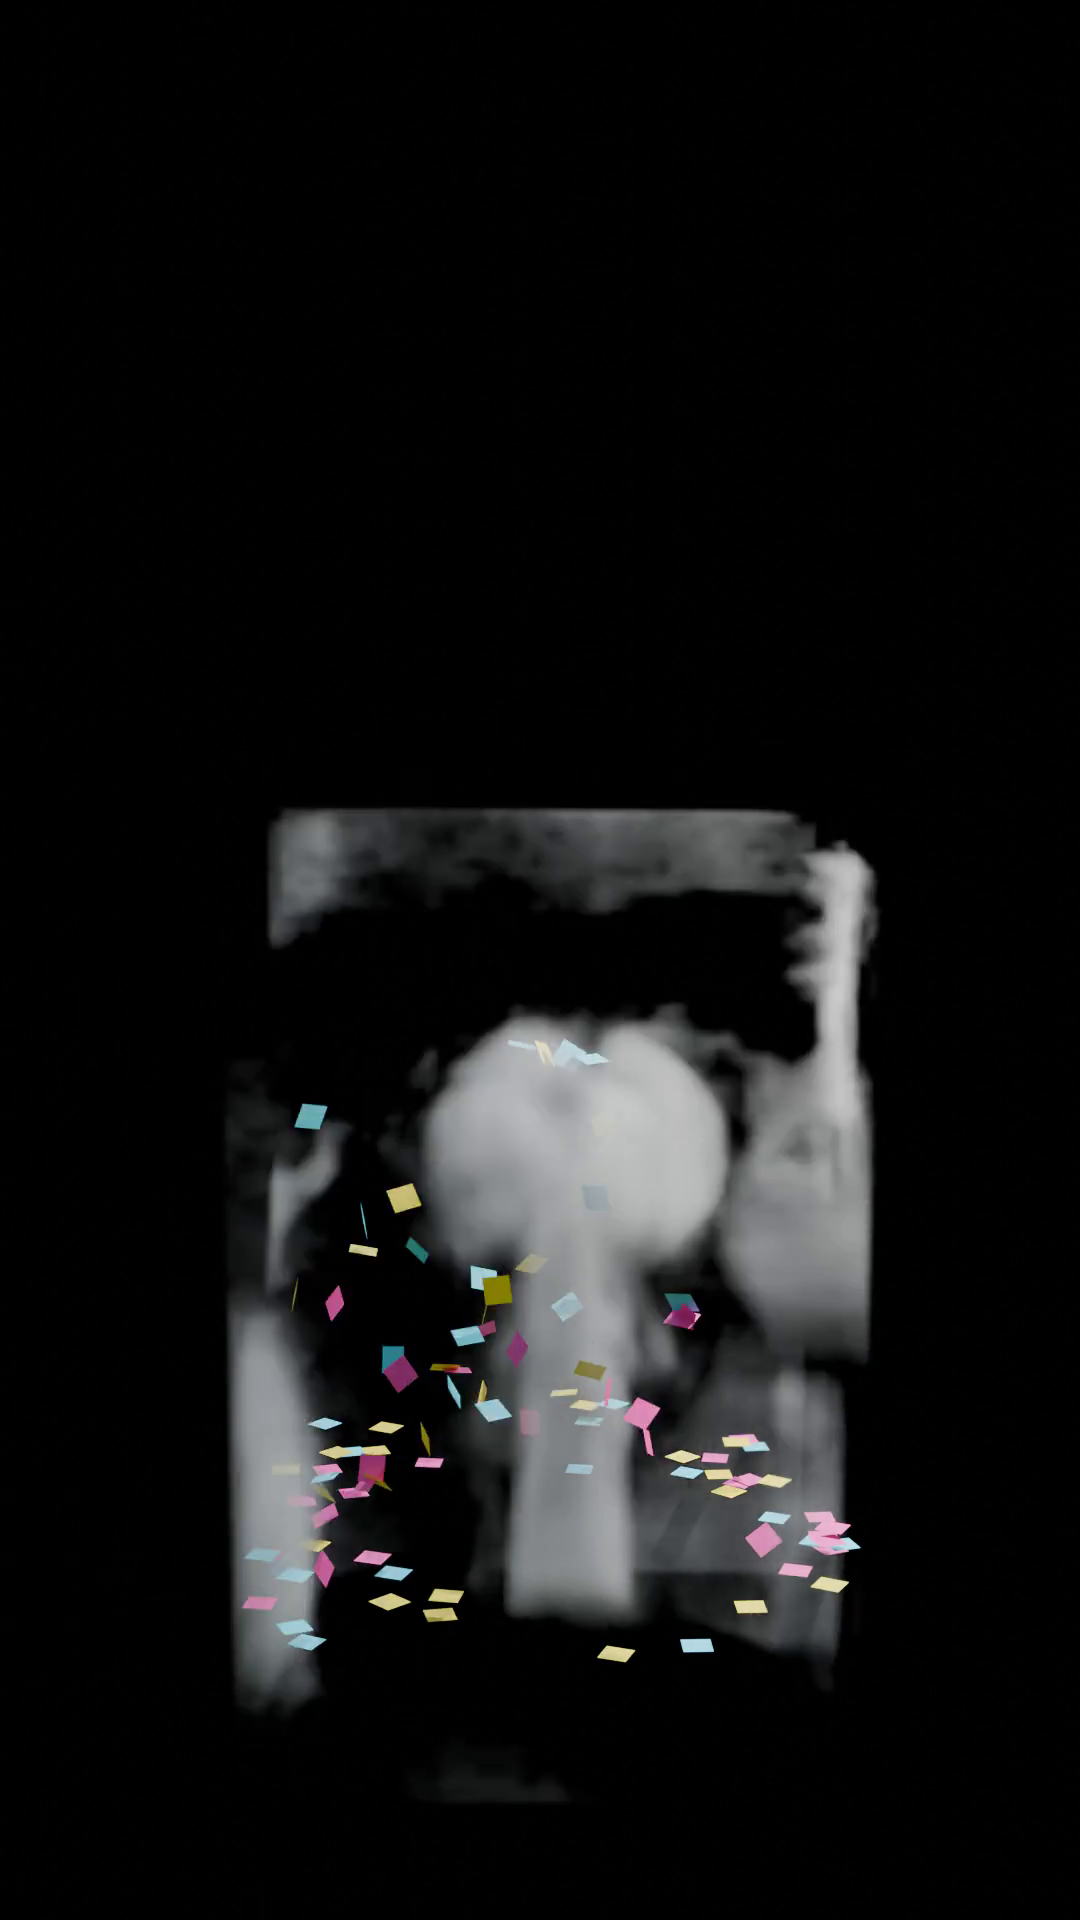}{\textbf{Hyfluid}}
    \hspace{-0.18cm}
    % \hfill
    % \formattedgraphics{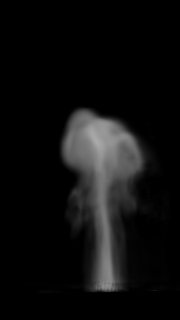}{Ours}%
    % \mygraphics{fig/Experiments/ScalarSyn_resim/029.png}{\textbf{Ours}}{PSNR $\vb{32.91}$}
    \formattedgraphics{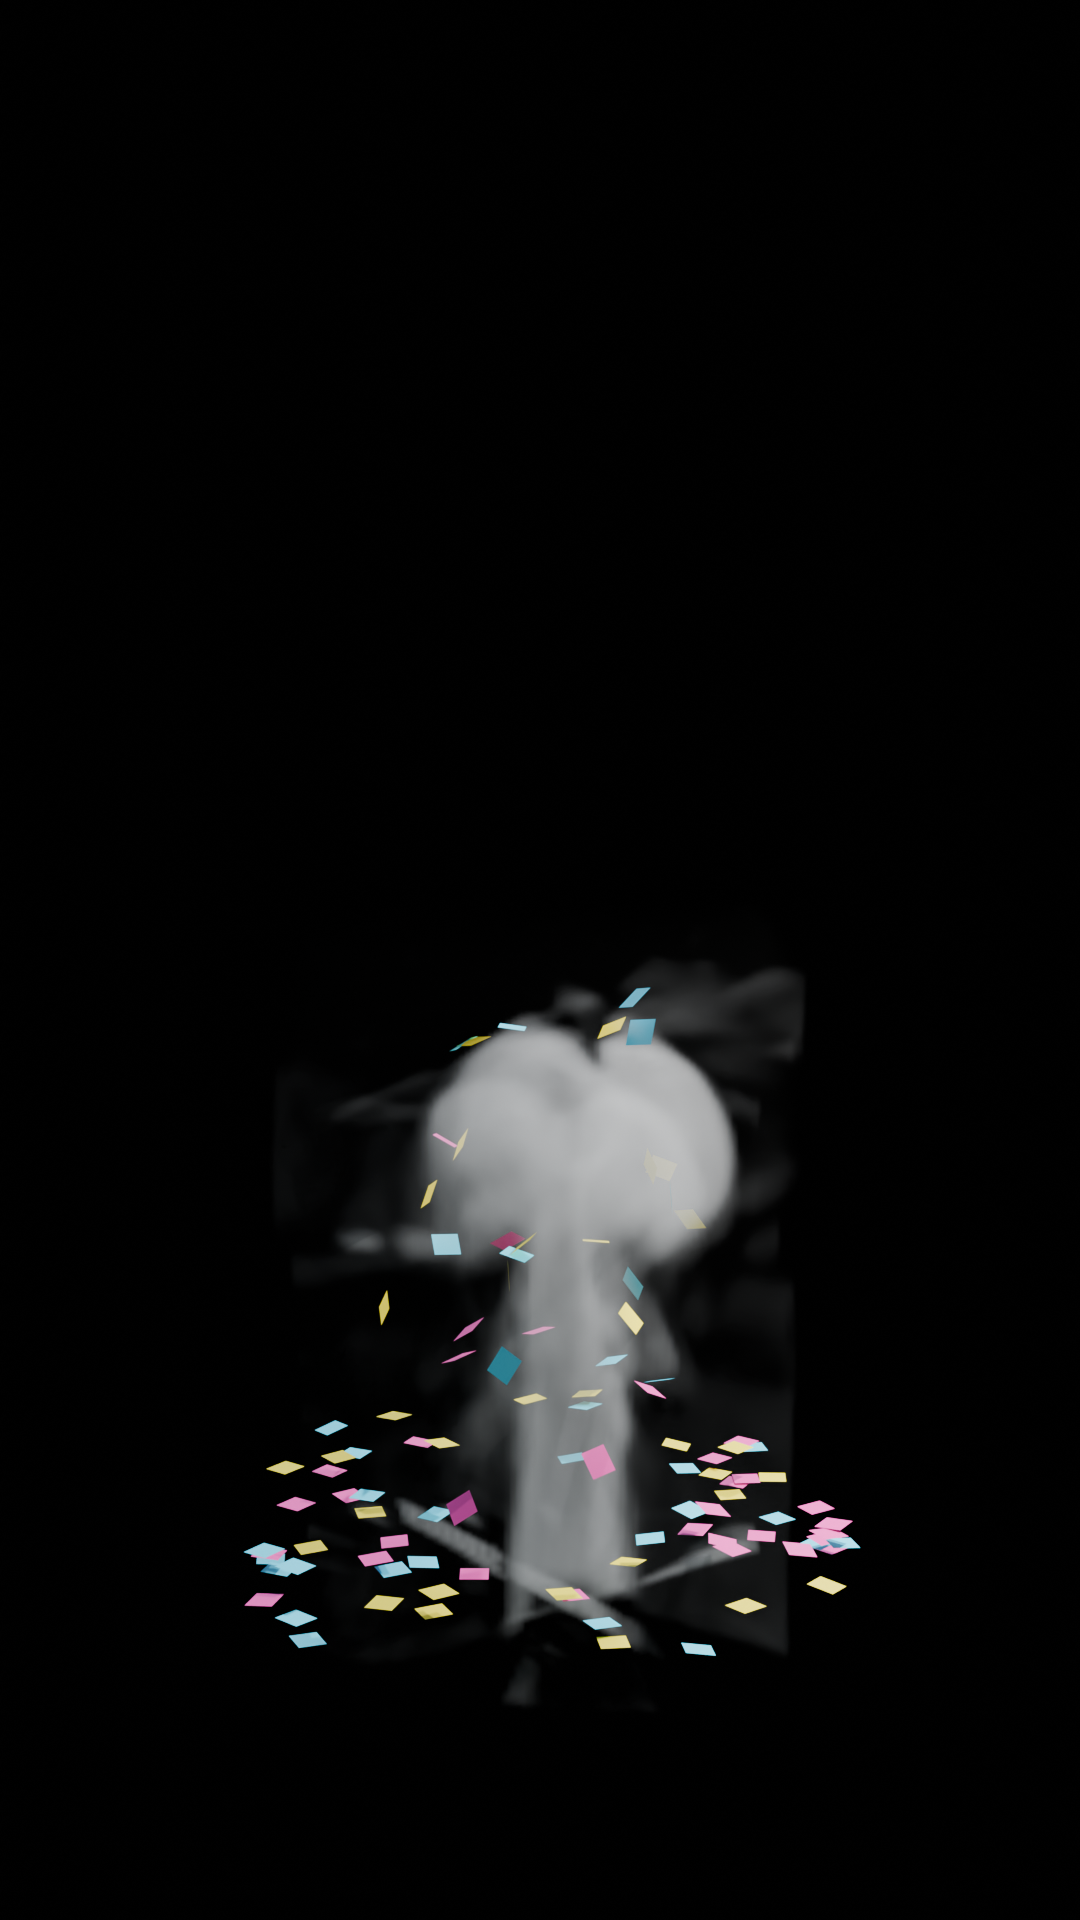}{\textbf{Ours}}
    \hspace{-0.18cm}
    % \hfill
    % \formattedgraphics{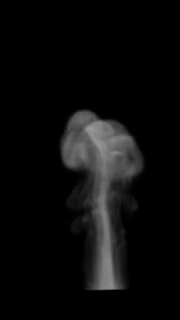}{\textbf{Ground Truth}}%
    \formattedgraphics{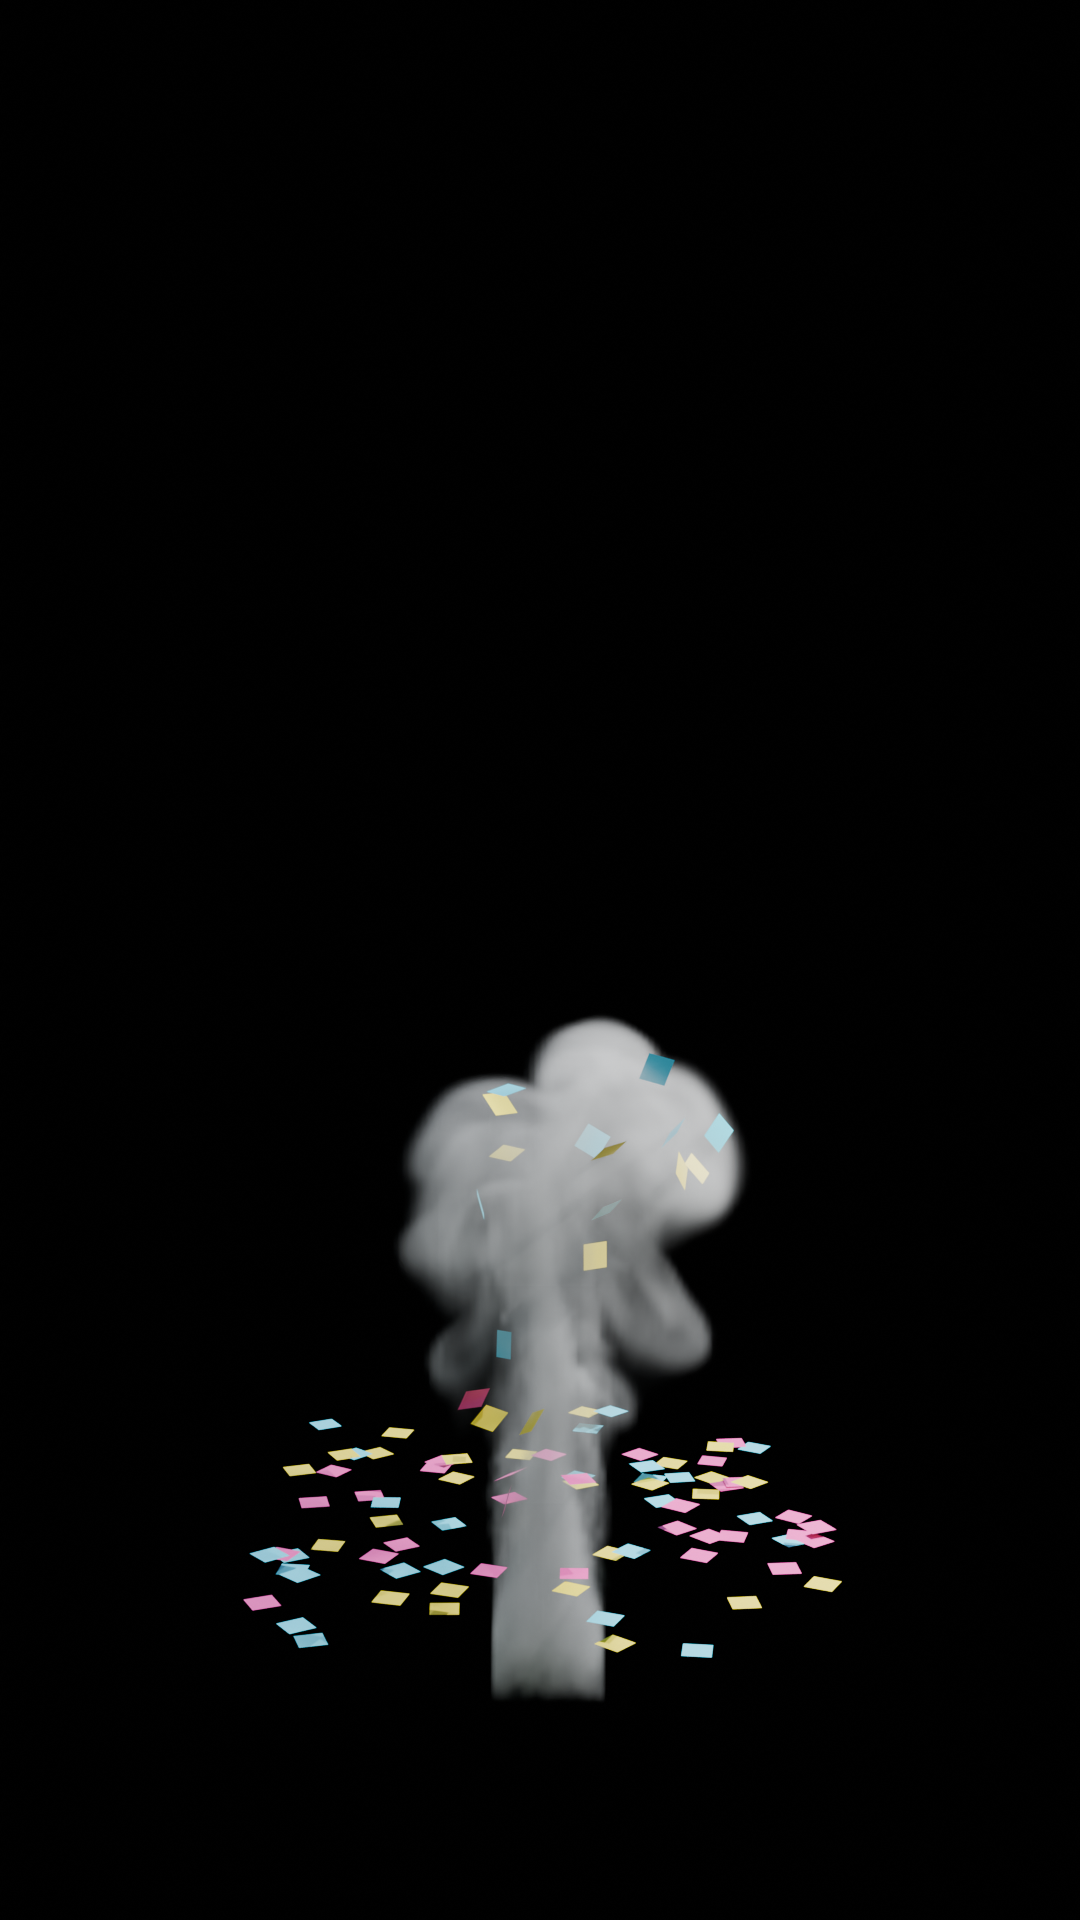}{\textbf{Ground Truth}}
    \\
    \vspace{-6pt}
    \caption{\rv{Tracer visualization results on the ScalarSyn scene, where the reconstructed velocity from baseline methods is masked using the ground truth density with a threshold of $0$. With such a low threshold, the baseline velocity field lifts paper pieces that should remain stationary.}}
    \label{fig:tracerThresh0}
  \end{figure*}

\begin{figure*}[htbp]
    \centering
    \setlength{\imagewidth}{0.2\textwidth}
      \newcommand{\formattedgraphics}[2]{%
        \begin{tikzpicture}%[spy using outlines={rectangle, magnification=2, connect spies}]
          \clip (0, 15pt) rectangle (\imagewidth, 140pt);
          \node[anchor=south west, inner sep=0] at (0,0){\includegraphics[width=\imagewidth,trim={3cm 0cm 3cm 7cm},clip]{#1}};
          %\spy [red,size=.41\imagewidth] on (0.65\imagewidth,1.05\imagewidth) in node at (0.25\imagewidth,.4\imagewidth);
          \node[anchor=west,text=white] at (.01\imagewidth, 1.27\imagewidth) {\sffamily\footnotesize #2};
          \end{tikzpicture}%
      }
      \newcommand{\mygraphics}[3]{%
        \begin{tikzpicture}[spy using outlines={rectangle, magnification=2, connect spies}]
          \clip (0, 15pt) rectangle (\imagewidth, 140pt);
          \node[anchor=south west, inner sep=0] at (0,0){\includegraphics[width=\imagewidth]{#1}};
          \spy [red,size=.41\imagewidth] on (0.65\imagewidth,1.05\imagewidth) in node at (0.25\imagewidth,.4\imagewidth);
          \node[anchor=west,text=white] at (.01\imagewidth, 1.29\imagewidth) {\sffamily\footnotesize #2};
          \node[anchor=west,text=white] at (0.01\imagewidth, 1.205\imagewidth) {\sffamily\scriptsize #3};%
          \end{tikzpicture}%
      }
    % \formattedgraphics{fig/Experiments/ScalarSyn_resim/pinf_029.png}{PINF}%
    \formattedgraphics{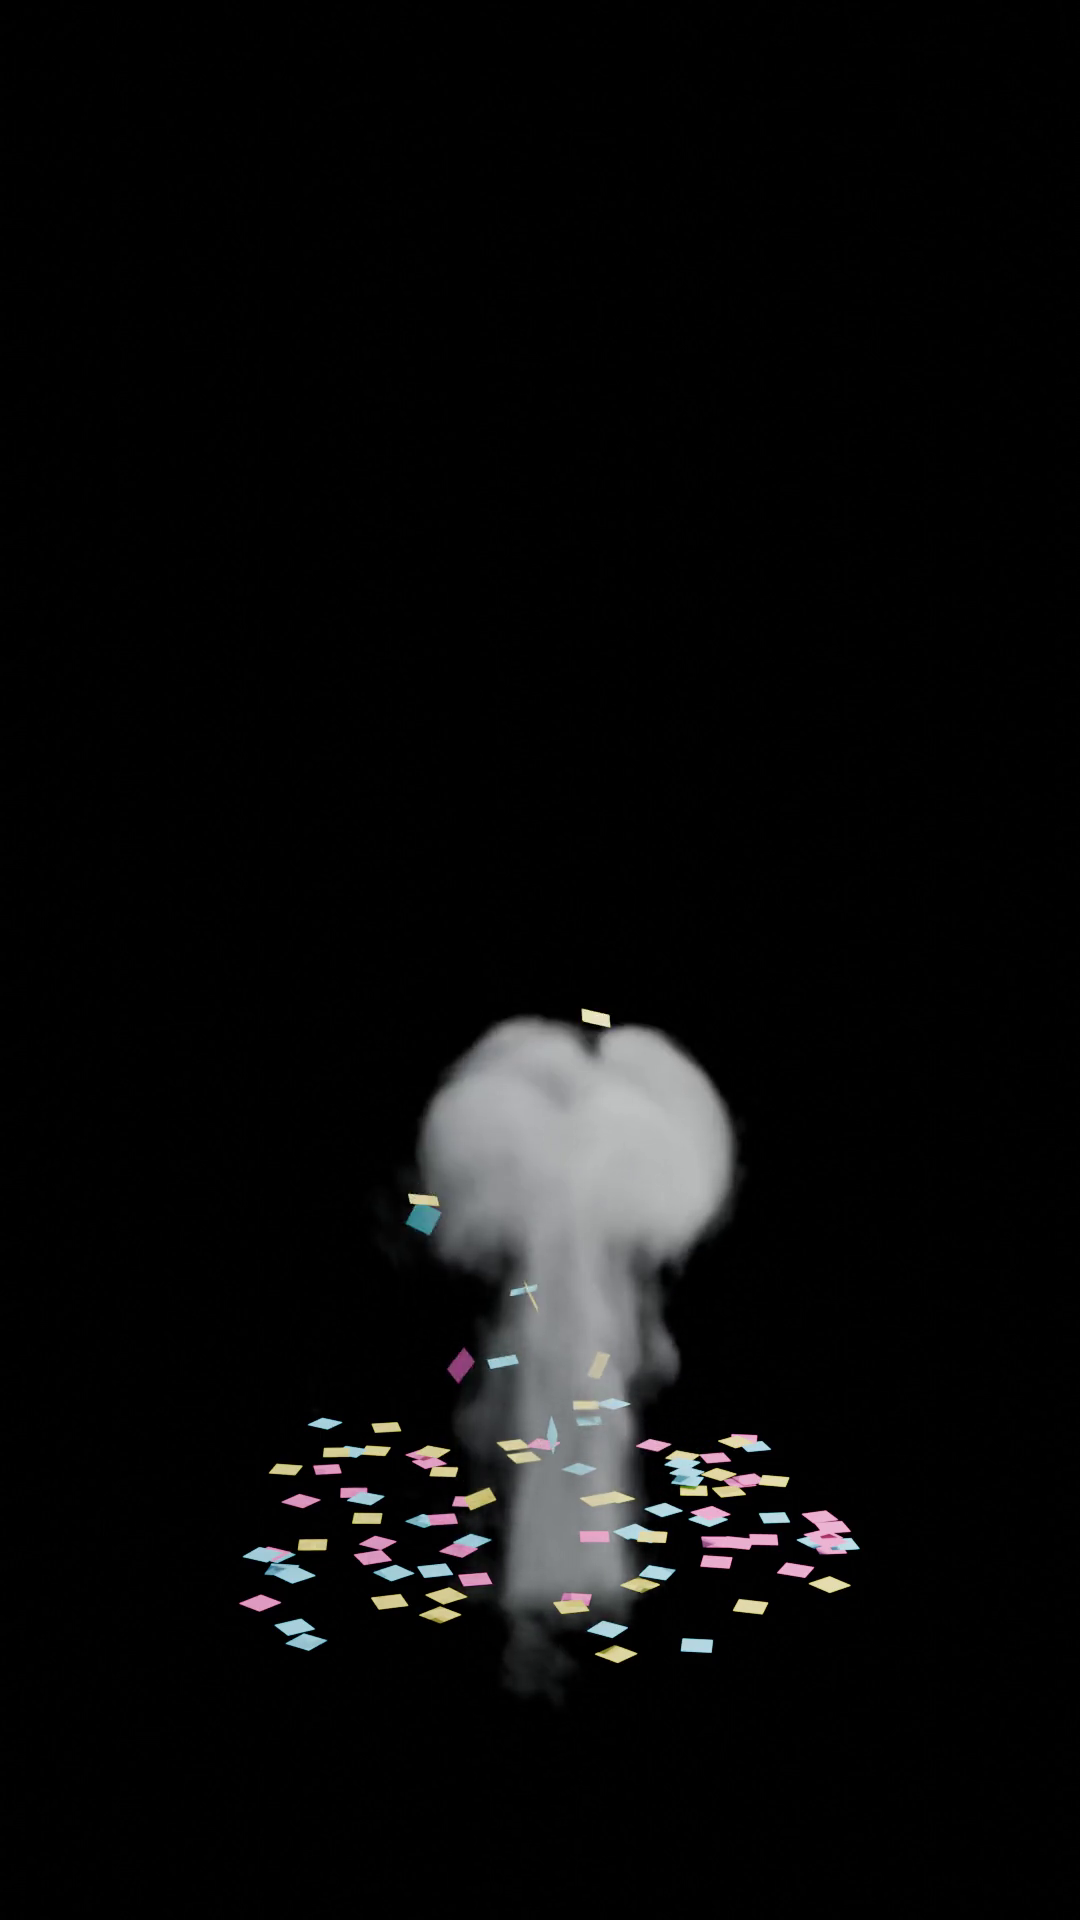}{\textbf{PINF}}
    \hspace{-0.18cm}
    % \hfill
    % \formattedgraphics{fig/Experiments/ScalarSyn_resim/pict_029.png}{PICT}%
    % \mygraphics{fig/Experiments/ScalarSyn_resim/pict_029.png}{\textbf{PICT}}{PSNR $31.00$}
    \formattedgraphics{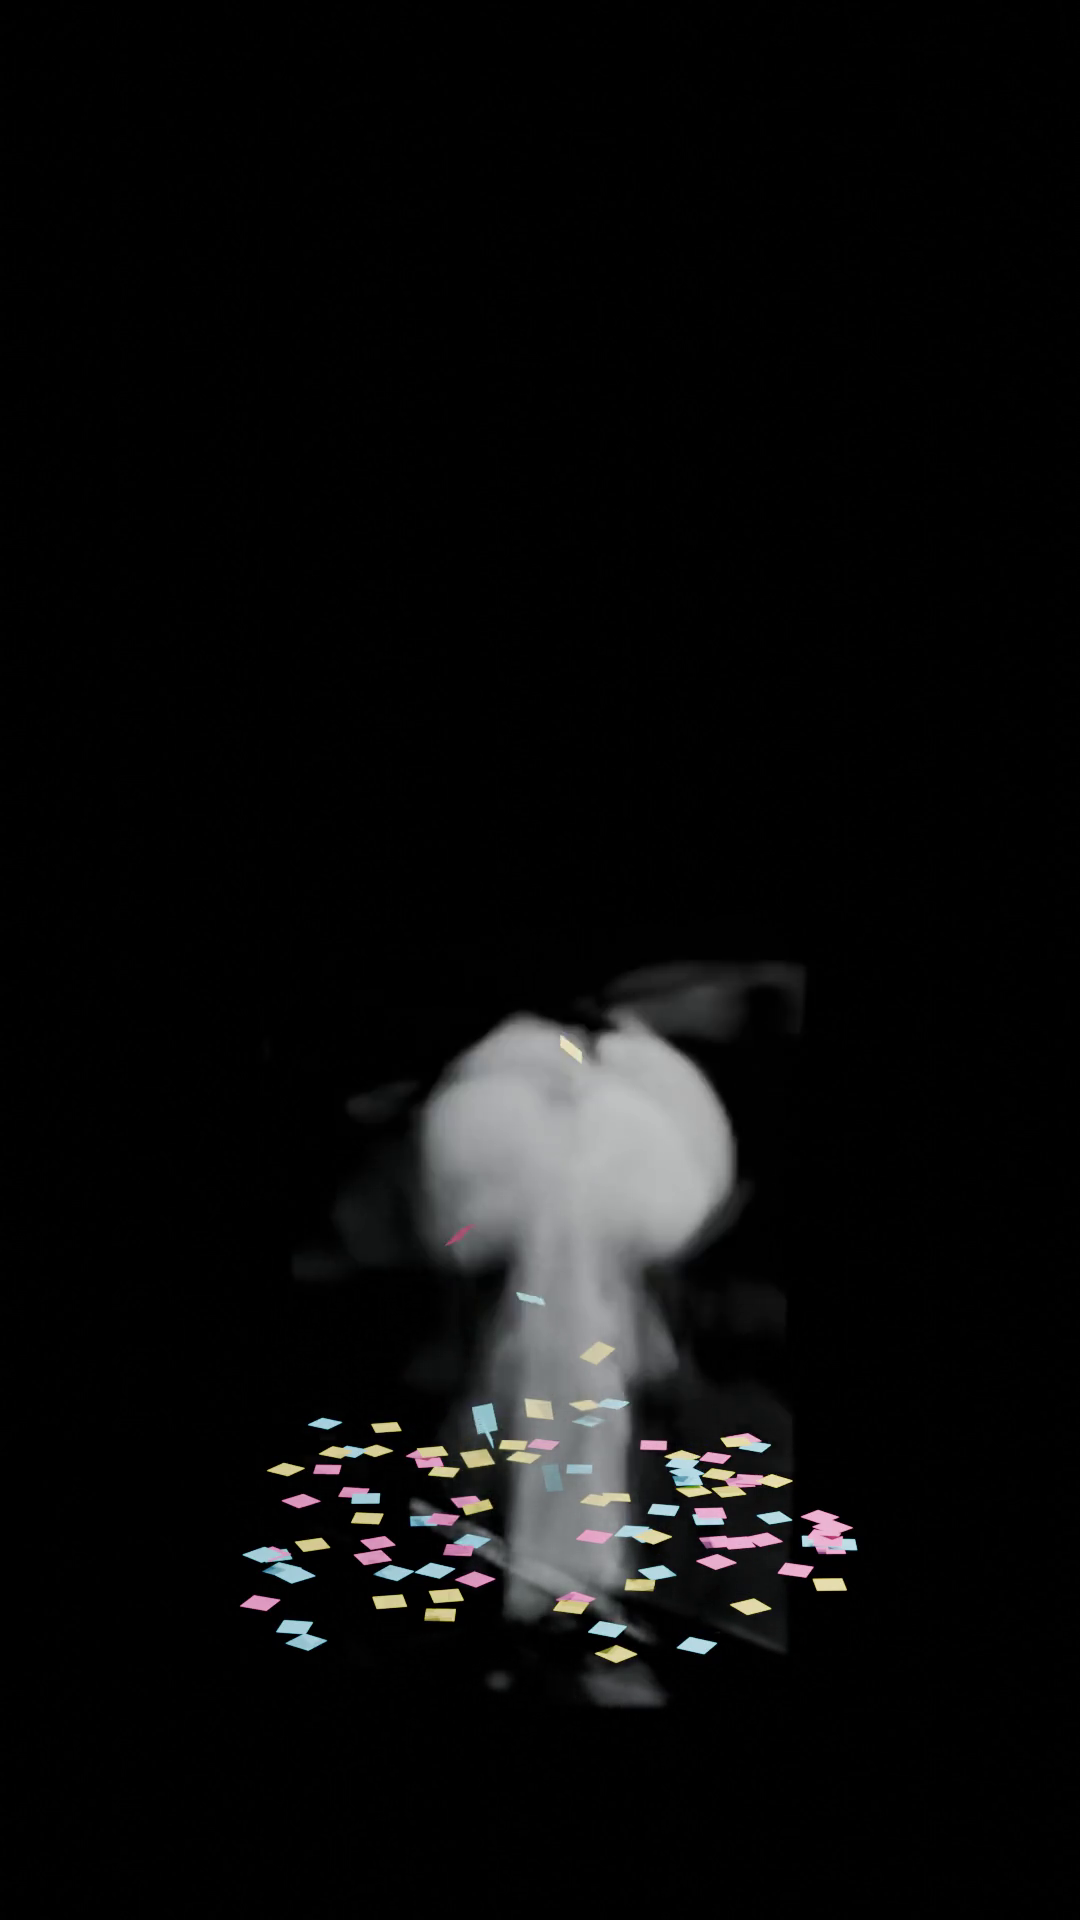}{\textbf{PICT}}
    \hspace{-0.18cm}
    % \hfill
    % \formattedgraphics{fig/Experiments/ScalarSyn_resim/HyFluid_rgb_029.png}{HyFluid}%
    % \mygraphics{fig/Experiments/ScalarSyn_resim/HyFluid_rgb_029.png}{\textbf{Hyfluid}}{PSNR $32.41$}
    \formattedgraphics{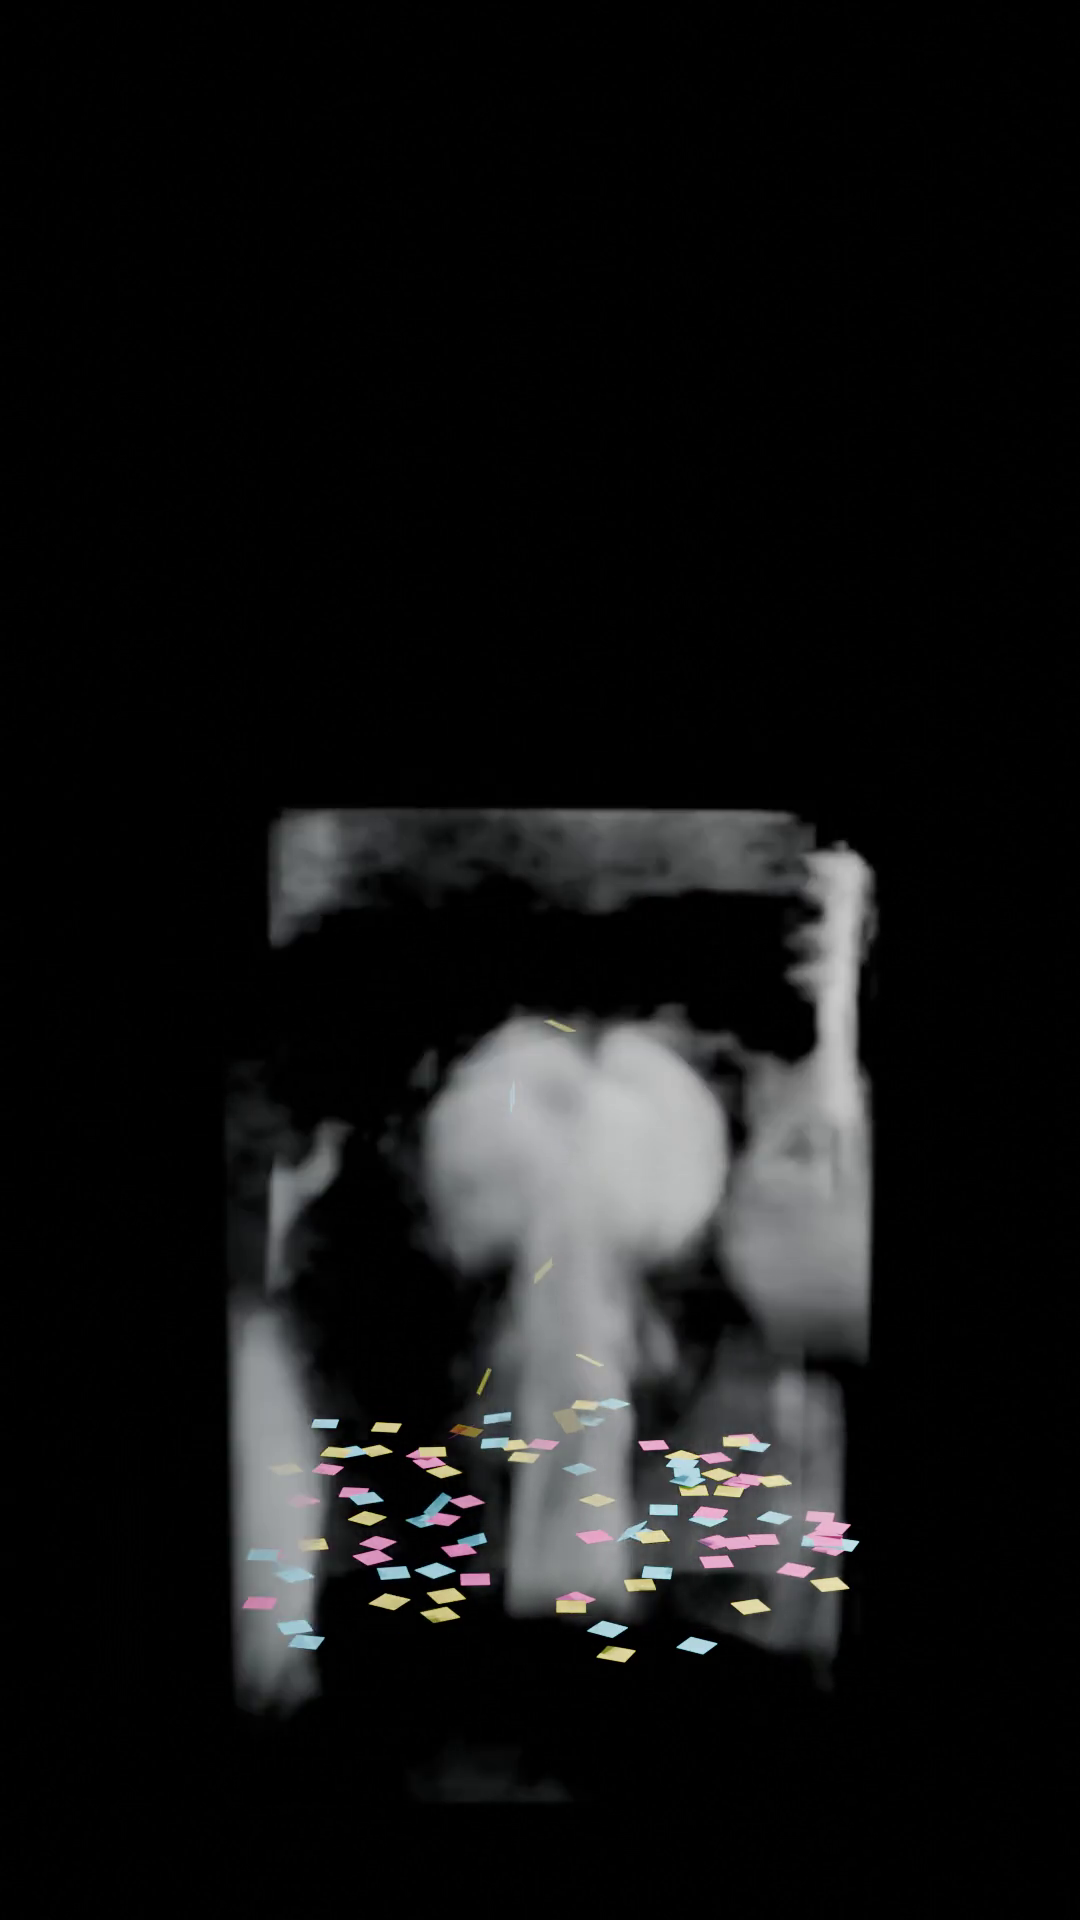}{\textbf{Hyfluid}}
    \hspace{-0.18cm}
    % \hfill
    % \formattedgraphics{fig/Experiments/ScalarSyn_resim/029.png}{Ours}%
    % \mygraphics{fig/Experiments/ScalarSyn_resim/029.png}{\textbf{Ours}}{PSNR $\vb{32.91}$}
    \formattedgraphics{fig/Experiments/tracer/ours_syn_0029.png}{\textbf{Ours}}
    \hspace{-0.18cm}
    % \hfill
    % \formattedgraphics{fig/Experiments/ScalarSyn_resim/gt_029.png}{\textbf{Ground Truth}}%
    \formattedgraphics{fig/Experiments/tracer/gt_syn_0029.png}{\textbf{Ground Truth}}
    \\
    \vspace{-6pt}
    \caption{\rv{Tracer visualization results on the ScalarSyn scene, where the reconstructed velocity from baseline methods is masked using the ground truth density with a threshold of $1$. As seen in the figure, a high threshold allows only a few paper pieces to be lifted compared to the ground truth.}}
    \label{fig:tracerThresh1}
  \end{figure*}

\rv{
\subsection{Comparison with FluidNexus}
\label{sec:fluidnexus}
We also compare our approach with FluidNexus~\cite{gao2025fluidnexus}. FluidNexus employs a Two-layer Particle Fluid Representation: a particle-based fluid (PBF) layer to enforce physical constraints, and a 3D Gaussian Splatting (3DGS) layer for rendering. Their method transforms multi-view reconstruction into a single-view problem by introducing a novel-view video synthesizer. Since our method focuses primarily on accurately reconstructing the velocity field, rather than on video generation, we evaluate both methods in multi-view mode on the ScalarFlow dataset~\cite{eckert2019scalar}.

As shown in Fig.~\ref{fig:velcmpFluidNexus}, we visualize the reconstructed velocity fields with the same visualization approach as in \S\ref{sec:analysis}. For FluidNexus, we adopt their kernel-weighted interpolation scheme to compute velocities at each grid center. Qualitative results show that the PBF representation struggles to capture the high-frequency details of the fluid. Furthermore, we compare the average divergence of the reconstructed velocities, which indicates that our PDE-based physical constraints produce more physically plausible results.

We also evaluate the re-simulation task (Fig.~\ref{fig:resimCmpFluidNexus}). Since the re-simulation code for FluidNexus is not publicly available, we implement it by advecting the 3DGS particles using the PBF-represented velocities at each frame. The results show that, although FluidNexus preserves the overall structure of the smoke, its output remains relatively coarse compared to ours.
}

\begin{figure}[bp]
    \centering
    \begin{minipage}[t]{0.8\linewidth}
        \centering
        \begin{minipage}[t]{\linewidth}
            %\centering
            \includegraphics[width=\linewidth]{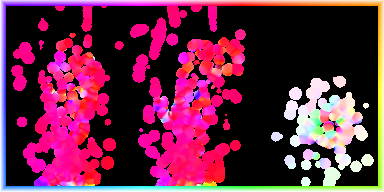}
            \vspace{-20pt}
            \caption*{\textbf{FluidNexus}\\{\small Divergence $0.04068$}}
            % \caption*{\textbf{FluidNexus} (divergence$\downarrow$ $0.04068$)}
            \includegraphics[width=\linewidth]{fig/Experiments/ScalarReal_vel/hfreq_vel_image_000110.png}
            \vspace{-20pt}
            \caption*{\textbf{Ours}\\{\small Divergence $\mathbf{0.0004503}$}}
            % \caption*{\textbf{Ours} (divergence$\downarrow$ $0.0004503$)}

        \end{minipage}%
        % \hfill
    \end{minipage}
    \vspace{-6pt}
    \caption{\rv{Velocity comparison with FluidNexus on the ScalarFlow dataset. From the results, it is clear that FluidNexus struggles to capture the high-frequency details of the velocity field, and its PBF representation imposes weaker physical constraints than our PDE-based approach, resulting in a larger divergence.}}
    \label{fig:velcmpFluidNexus}
\end{figure}

\begin{figure}[t]
    \centering
    \setlength{\imagewidth}{0.325\linewidth}
      \newcommand{\formattedgraphics}[2]{%
        \begin{tikzpicture}
        \clip (0, 5pt) rectangle (\imagewidth, 120pt); 
          \node[anchor=south west, inner sep=0] at (0,0){\includegraphics[width=\imagewidth]{#1}};
          %\draw[red] (0.25\imagewidth, 0.2\imagewidth) rectangle (0.7\imagewidth, 0.65\imagewidth);
          \node[anchor=west,text=white] at (.01\imagewidth, 1.4\imagewidth) {\sffamily\footnotesize #2};
          \end{tikzpicture}%
      }
      \newcommand{\mygraphics}[3]{%
        \begin{tikzpicture}
        \clip (0, 5pt) rectangle (\imagewidth, 120pt); 
          \node[anchor=south west, inner sep=0] at (0,0){\includegraphics[width=\imagewidth]{#1}};
          %\draw[red] (0.25\imagewidth, 0.2\imagewidth) rectangle (0.7\imagewidth, 0.65\imagewidth);
          \node[anchor=west,text=white] at (.01\imagewidth, 1.4\imagewidth) {\sffamily\footnotesize #2};
          \node[anchor=west,text=white] at (.01\imagewidth, 1.28\imagewidth) {\sffamily\scriptsize #3};
          \end{tikzpicture}%
      }
    % \formattedgraphics{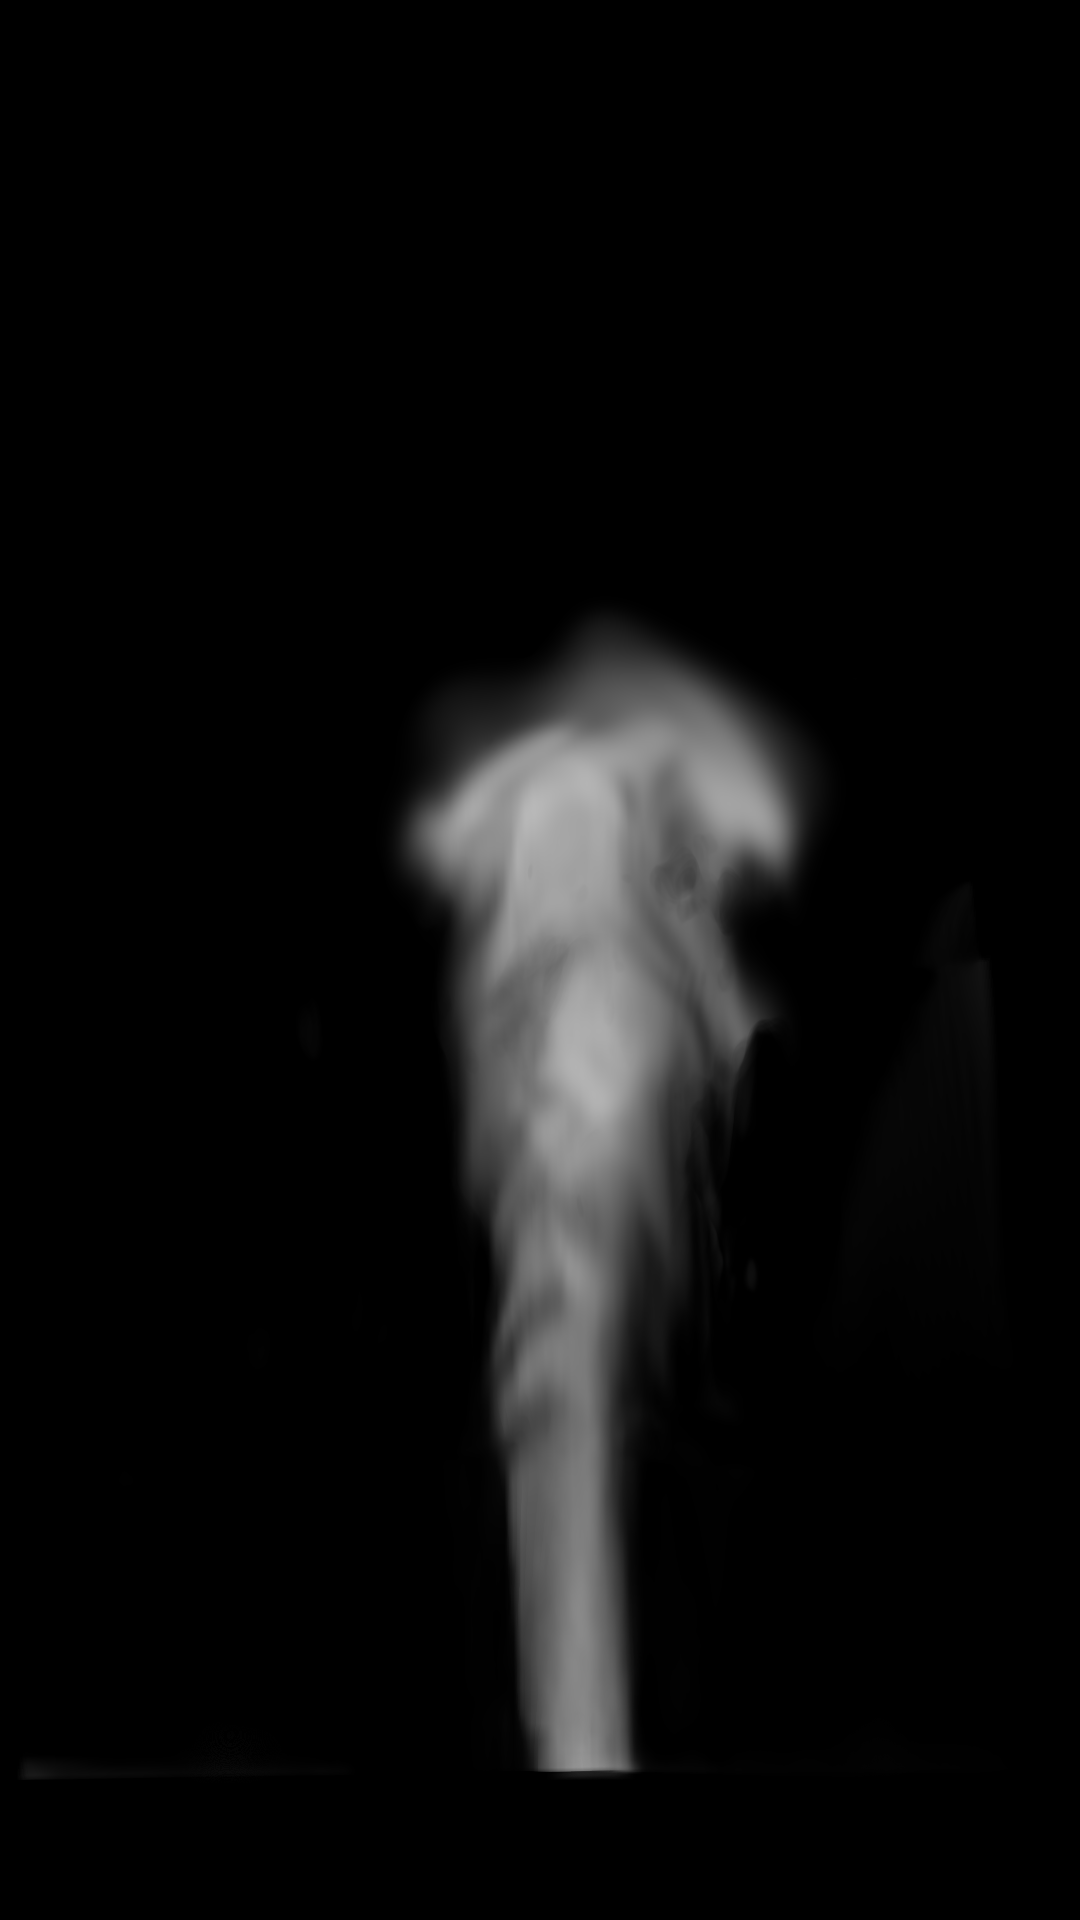}{Coarse-level}
    \mygraphics{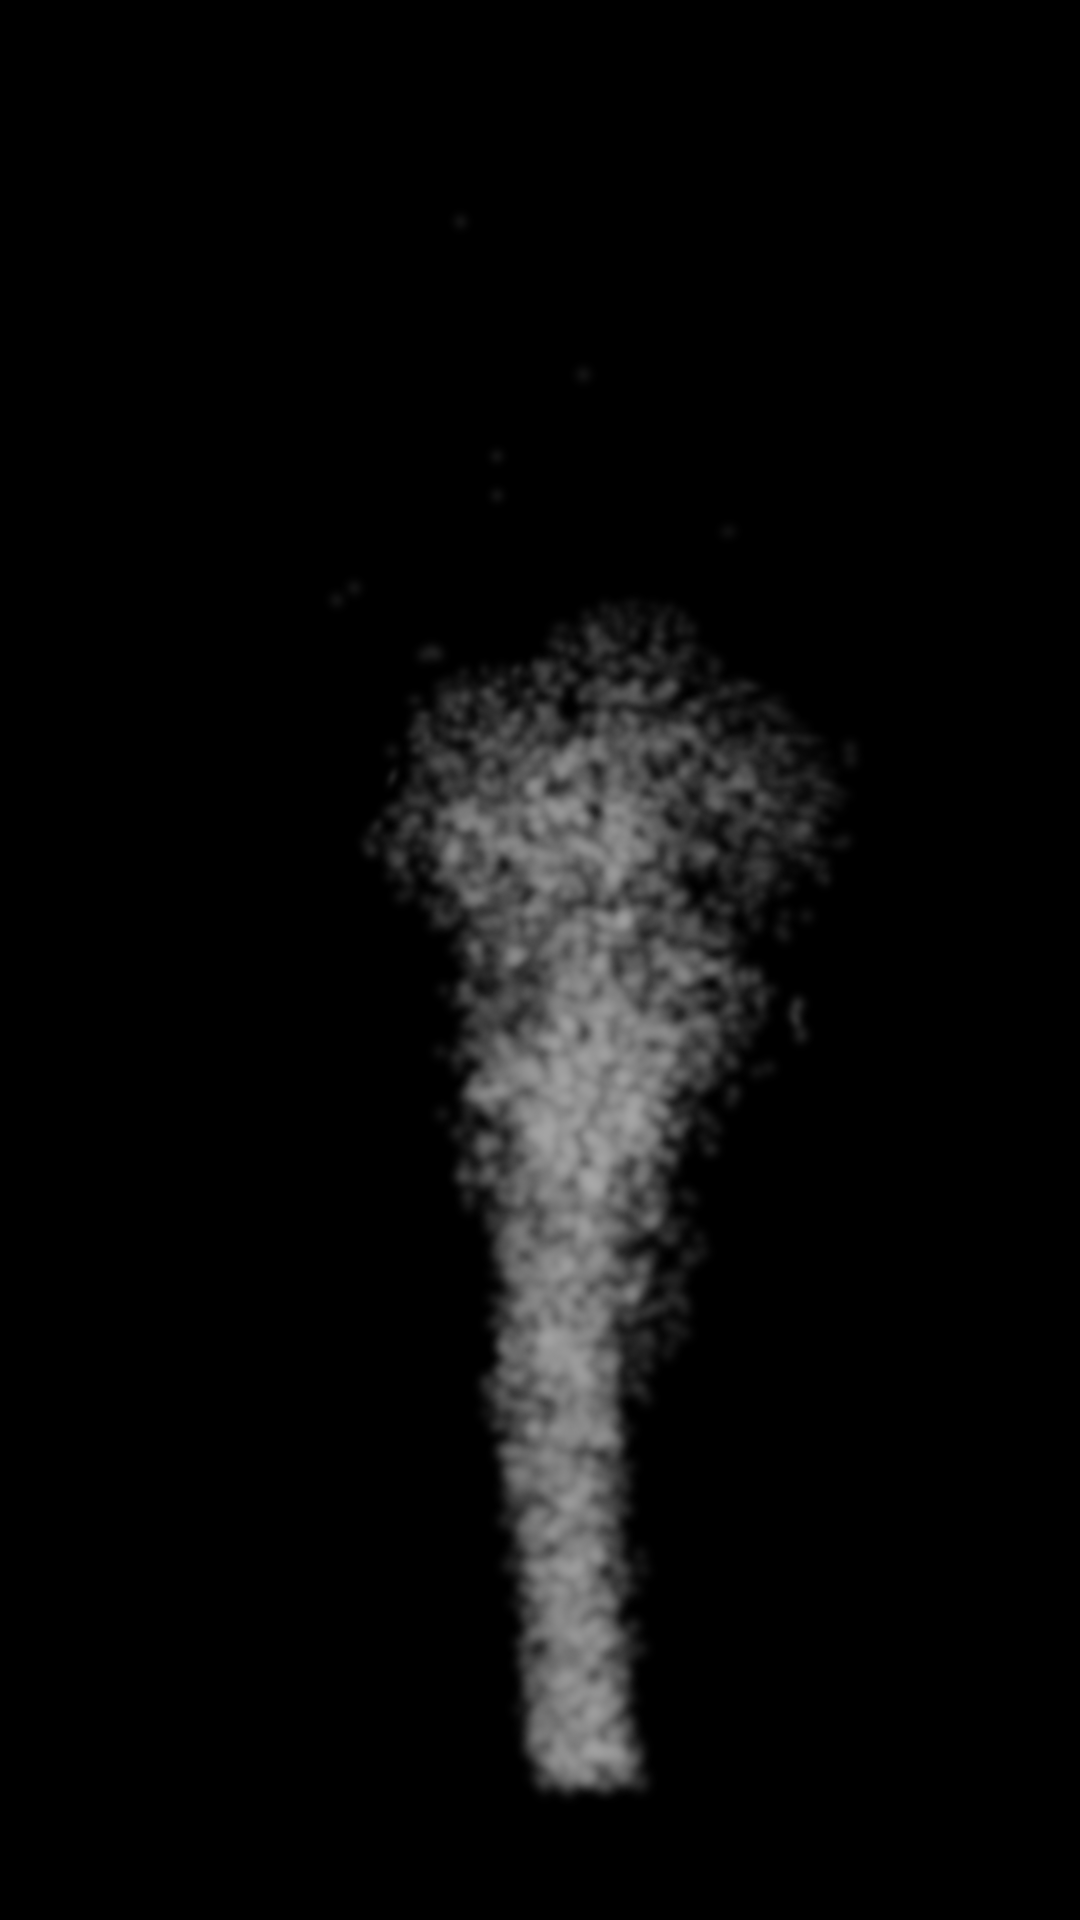}{\textbf{FluidNexus}}{PSNR $30.99$}
    \hspace{-0.2cm}
 % \formattedgraphics{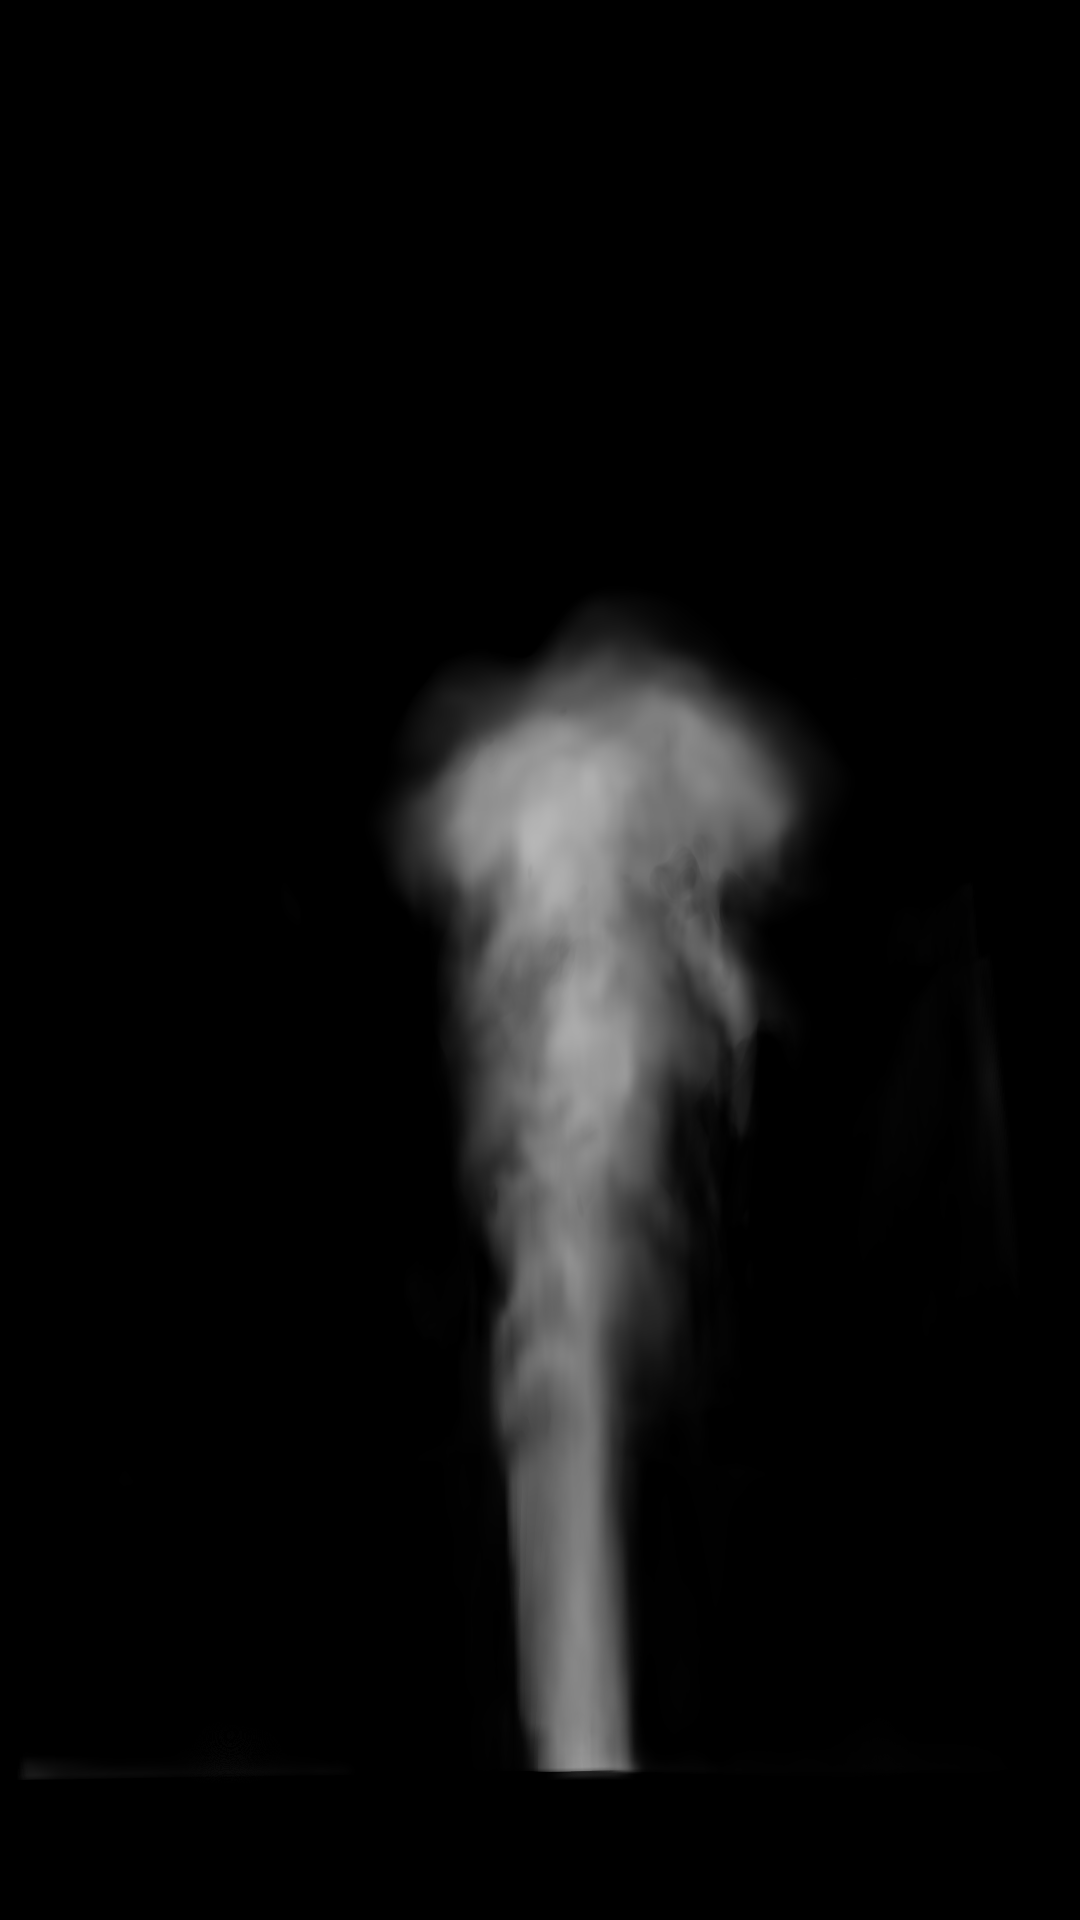}{Full}
 \mygraphics{fig/Experiments/Ablation/add_hfreq_119.png}{\textbf{Ours}}{PSNR $\mathbf{33.28}$}
 \hspace{-0.2cm}
 \formattedgraphics{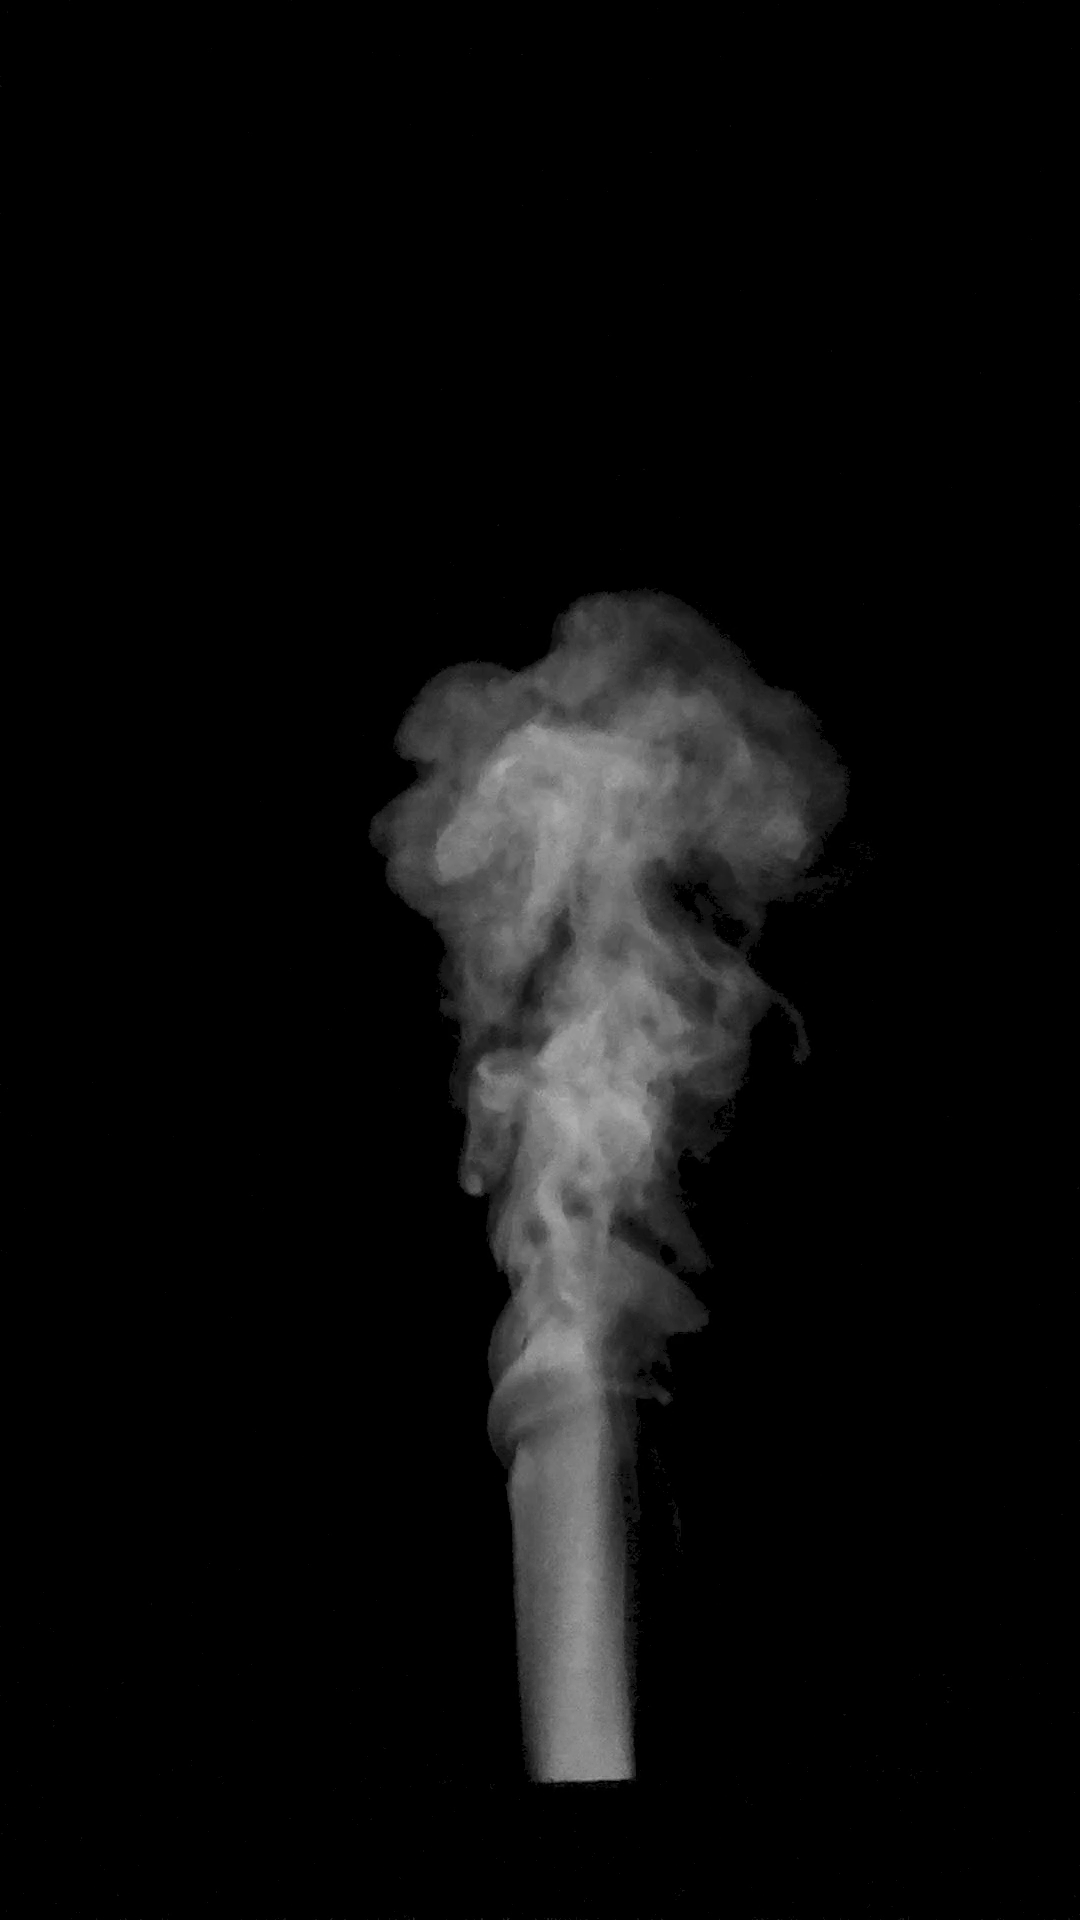}{\textbf{Ground Truth}}
    \\
    \vspace{-0.5em}
    \caption{\rv{Re-simulation results compared with FluidNexus on the ScalarFlow dataset. It can be seen that, although FluidNexus captures the overall structure of the smoke, it fails to reconstruct fine details, resulting in a lower PSNR value than ours.}}
    \label{fig:resimCmpFluidNexus}
  \end{figure}

\subsection{Implementation Details}
\paragraph{Model architecture}
For the density model, we follow~\citet{wang2024physics} and adopt a \emph{SIREN+T} model for the dynamic density and a NeuS~\cite{wang2021neus} model for the static boundary. For the coarse-level velocity representation, we employ a \emph{SIREN+T} model with $6$ hidden layers, each with a width of $128$. For the fine-level velocity representation, we use a 4D extension of iNGP~\cite{M_ller_2022,yu2024inferring}. Both the spatial and temporal components are encoded using multiresolution hash grids, with a base resolution of $128$ and a finest resolution of $512$, enabling the model to capture high-frequency details effectively.

\paragraph{Training and hyper-parameters}
Our training process consists of three stages. In the first stage, we train the density model using the settings described in the first-stage training of~\citet{wang2024physics}. In the second stage, we jointly train the density and coarse-level velocity, where the loss weights are set as follows: $\lambda_{\text{vor}} = 10^{-5}$, $\lambda_{\text{div}} = 5 \times 10^{-3}$, $\lambda_{\text{kine}} = 10$, and $\lambda_{\text{bnd}} = 1000$. The transport loss $\mathcal{L}_{\text{trans}}$ uses 5 recursive advection steps with a discount factor $\beta = 0.95$. For the Cylinder scene, where the velocity is relatively weak, we reduce $\lambda_{\text{kine}}$ and $\lambda_{\text{bnd}}$ to 1 and 100, respectively, to avoid suppressing the velocity field. In the third stage, we train the fine-level velocity with $\lambda_{\text{warp}} = 1$ and $\lambda_{\text{proj}} = 10^6$. Both the second and third stages use the Adam optimizer with a learning rate of $10^{-3}$.
